# Supplementary material for: Perceptions of Sentient AI and Other Digital Minds: Evidence from the AI, Morality, and Sentience (AIMS) Survey
Source: arXiv:2407.08867 source file (2025-03-10)
Supplement: Supplementary file 1 [file Main_Survey_-_Participant_View.pdf]

Thank you for participating in this survey. Your honest responses will help researchers better understand public perceptions of artificial intelligence and robots. We would like a truthful understanding of your perspective. There are no right or wrong answers.

There are no known or anticipated risks to you for participating. Although this study will not benefit you personally, it may be interesting and we hope that our results will help us understand how people think about artificial intelligence. Participation will take approximately 15 minutes. All of your responses will be anonymous.

**We will ask questions to ensure you are paying attention, and you cannot go back in this survey, so please take your time before answering.**

**By clicking the 'Next' button you are giving your consent to take part in the survey.**

Next

---

Please take some time to read through the following definitions that will come up in this survey.

- **Artificial beings** and **robots/AIs** are **intelligent entities built by humans**, such as robots, virtual copies of human brains, or computer programs that solve problems, **with or without a physical body**, that may exist now or in the future.
- **Sentience** is the capacity to have positive and negative experiences, such as happiness and suffering.
- **Sentient robots/AIs** are those with the capacity to have positive and negative experiences, such as happiness and suffering.

Next

---

*Definition Reminder:*

- **Artificial beings** and **robots/AIs** are intelligent entities built by humans, such as robots, virtual copies of human brains, or computer programs that solve problems, with or without a physical body, that may exist now or in the future.
- **Sentience** is the capacity to have positive and negative experiences, such as happiness and suffering.
- **Sentient robots/AIs** are those with the capacity to have positive and negative experiences, such as happiness and suffering.

**To what extent do you agree or disagree with the following statements? (1 = strongly agree, 6 = strongly disagree)**

The welfare of robots/AIs is one of the most important social issues in the world today.

- (1) strongly agree
- (2) agree
- (3) somewhat agree
- (4) somewhat disagree
- (5) disagree
- (6) strongly disagree
- No opinion

Physically damaging sentient robots/AIs without their consent is wrong.

- (1) strongly agree
- (2) agree
- (3) somewhat agree
- (4) somewhat disagree
- (5) disagree
- (6) strongly disagree
- No opinion

Re-programming sentient robots/AIs without their consent is wrong.

- (1) strongly agree
- (2) agree
- (3) somewhat agree
- (4) somewhat disagree
- (5) disagree
- (6) strongly disagree
- No opinion

Torturing sentient robots/AIs is wrong.

- (1) strongly agree
- (2) agree
- (3) somewhat agree
- (4) somewhat disagree
- (5) disagree
- (6) strongly disagree
- No opinion

Sentient robots/AIs deserve to be included in the moral circle.

- (1) strongly agree
- (2) agree
- (3) somewhat agree
- (4) somewhat disagree
- (5) disagree
- (6) strongly disagree
- No opinion

Sentient robots/AIs deserve to be treated with respect.

- (1) strongly agree
- (2) agree
- (3) somewhat agree
- (4) somewhat disagree
- (5) disagree
- (6) strongly disagree
- No opinion

Next

*Definition Reminder:*

- **Artificial beings** and **robots/AIs** are intelligent entities built by humans, such as robots, virtual copies of human brains, or computer programs that solve problems, with or without a physical body, that may exist now or in the future.
- **Sentience** is the capacity to have positive and negative experiences, such as happiness and suffering.
- **Sentient robots/AIs** are those with the capacity to have positive and negative experiences, such as happiness and suffering.

**To what extent do you agree or disagree with the following statements? (1 = strongly agree, 6 = strongly disagree)**

I would consider joining a public demonstration against the mistreatment of sentient robots/AIs.

(1) strongly agree

(2) agree

(3) somewhat agree

(4) somewhat disagree

(5) disagree

(6) strongly disagree

No opinion

I support asking institutions like the government and private corporations to fund research that protects sentient robots/AIs.

- (1) strongly agree
- (2) agree
- (3) somewhat agree
- (4) somewhat disagree
- (5) disagree
- (6) strongly disagree
- No opinion

I support campaigns against the exploitation of sentient robots/AIs.

- (1) strongly agree
- (2) agree
- (3) somewhat agree
- (4) somewhat disagree
- (5) disagree
- (6) strongly disagree
- No opinion

Next

*Definition Reminder:*

- **Artificial beings** and **robots/AIs** are intelligent entities built by humans, such as robots, virtual copies of human brains, or computer programs that solve problems, with or without a physical body, that may exist now or in the future.
- **Sentience** is the capacity to have positive and negative experiences, such as happiness and suffering.
- **Sentient robots/AIs** are those with the capacity to have positive and negative experiences, such as happiness and suffering.

**To what extent do you agree or disagree with the following statements? (1 = strongly agree, 6 = strongly disagree)**

It is wrong to blackmail people by threatening to harm robots/AIs they care about.

(1) strongly agree

(2) agree

(3) somewhat agree

(4) somewhat disagree

(5) disagree

(6) strongly disagree

No opinion

Sentient robots/AIs deserve to be protected from people who derive pleasure from inflicting physical or mental pain on them.

- (1) strongly agree
- (2) agree
- (3) somewhat agree
- (4) somewhat disagree
- (5) disagree
- (6) strongly disagree
- No opinion

It is right to protect sentient robots/AIs from vindictive or retaliatory punishment.

- (1) strongly agree
- (2) agree
- (3) somewhat agree
- (4) somewhat disagree
- (5) disagree
- (6) strongly disagree
- No opinion

Next

*Definition Reminder:*

- **Artificial beings** and **robots/AIs** are intelligent entities built by humans, such as robots, virtual copies of human brains, or computer programs that solve problems, with or without a physical body, that may exist now or in the future.
- **Sentience** is the capacity to have positive and negative experiences, such as happiness and suffering.
- **Sentient robots/AIs** are those with the capacity to have positive and negative experiences, such as happiness and suffering.

**To what extent do you agree or disagree with the following statements? (1 = strongly agree, 6 = strongly disagree)**

I support a global ban on the development of applications that put the welfare of robots/AIs at risk.

(1) strongly agree

(2) agree

(3) somewhat agree

(4) somewhat disagree

(5) disagree

(6) strongly disagree

No opinion

I support a global ban on the development of sentience in robots/AIs.

- (1) strongly agree
- (2) agree
- (3) somewhat agree
- (4) somewhat disagree
- (5) disagree
- (6) strongly disagree
- No opinion

I support a global ban on the development of robot-human hybrids.

- (1) strongly agree
- (2) agree
- (3) somewhat agree
- (4) somewhat disagree
- (5) disagree
- (6) strongly disagree
- No opinion

I support a global ban on the development of AI-enhanced humans.

- (1) strongly agree
- (2) agree
- (3) somewhat agree
- (4) somewhat disagree
- (5) disagree
- (6) strongly disagree
- No opinion

Next

---

*Definition Reminder:*

- **Artificial beings** and **robots/AIs** are intelligent entities built by humans, such as robots, virtual copies of human brains, or computer programs that solve problems, with or without a physical body, that may exist now or in the future.
- **Sentience** is the capacity to have positive and negative experiences, such as happiness and suffering.
- **Sentient robots/AIs** are those with the capacity to have positive and negative experiences, such as happiness and suffering.

**To what extent do current robots/AIs (i.e., those that exist in 2021) have the capacity for each of the following (0 = not at all, 100 = very much)?**

having feelings

(0) not at all | Slide to answer | (100) very much

thinking analytically

(0) not at all | Slide to answer | (100) very much

experiencing emotions

(0) not at all | Slide to answer | (100) very much

being rational

(0) not at all | Slide to answer | (100) very much

Next

*Definition Reminder:*

- **Artificial beings** and **robots/AIs** are intelligent entities built by humans, such as robots, virtual copies of human brains, or computer programs that solve problems, with or without a physical body, that may exist now or in the future.
- **Sentience** is the capacity to have positive and negative experiences, such as happiness and suffering.
- **Sentient robots/AIs** are those with the capacity to have positive and negative experiences, such as happiness and suffering.

**To what extent do you agree or disagree with the following statements? (1 = strongly agree, 6 = strongly disagree)**

I support granting legal rights to sentient robots/AIs.

- (1) strongly agree
- (2) agree
- (3) somewhat agree
- (4) somewhat disagree
- (5) disagree
- (6) strongly disagree
- No opinion

I support the development of welfare standards that protect the well-being of sentient robots/AIs.

- (1) strongly agree
- (2) agree
- (3) somewhat agree
- (4) somewhat disagree
- (5) disagree
- (6) strongly disagree
- No opinion

I support a global ban on the use of sentient robots/AIs for labor without their consent.

- (1) strongly agree
- (2) agree
- (3) somewhat agree
- (4) somewhat disagree
- (5) disagree
- (6) strongly disagree
- No opinion

I support safeguards on scientific research practices that protect the well-being of sentient robots/AIs.

- (1) strongly agree
- (2) agree
- (3) somewhat agree
- (4) somewhat disagree
- (5) disagree
- (6) strongly disagree
- No opinion

I support a global ban on the use of sentient robots/AIs as subjects in medical experiments without their consent.

(1) strongly agree

(2) agree

(3) somewhat agree

(4) somewhat disagree

(5) disagree

(6) strongly disagree

No opinion

Next

---

**How much moral concern do you think you should show for the following robots/AIs? (1 = less concern, 5 = more concern)**

virtual avatars

who exist only in virtual space

(1) less concern — Slide to answer — (5) more concern

complex language algorithms

who learn and produce text from data

(1) less concern — Slide to answer — (5) more concern

machine-like factory production robots

who build parts for industry

(1) less concern

Slide to answer

(5) more concern

animal-like companion robots

who socialize with people at home

(1) less concern

Slide to answer

(5) more concern

AI personal assistants

who organize, schedule, and assist people in their daily lives

(1) less concern

Slide to answer

(5) more concern

machine-like cleaning robots

who clean people's spaces

(1) less concern

Slide to answer

(5) more concern

human-like retail robots

who interact with people at stores and restaurants

(1) less concern

Slide to answer

(5) more concern

exact digital copies of human brains

who exist in virtual space

(1) less concern

Slide to answer

(5) more concern

## human-like companion robots

who socialize with people at home

(1) less concern — Slide to answer — (5) more concern

## exact digital copies of animals

who exist in virtual space

(1) less concern — Slide to answer — (5) more concern

## AI video game characters

who exist only in video games

(1) less concern — Slide to answer — (5) more concern

Next

---

**On the following pages you will see circles like these. Please indicate which pair of circles best represents how connected you think the following robots/AIs are to humans.**

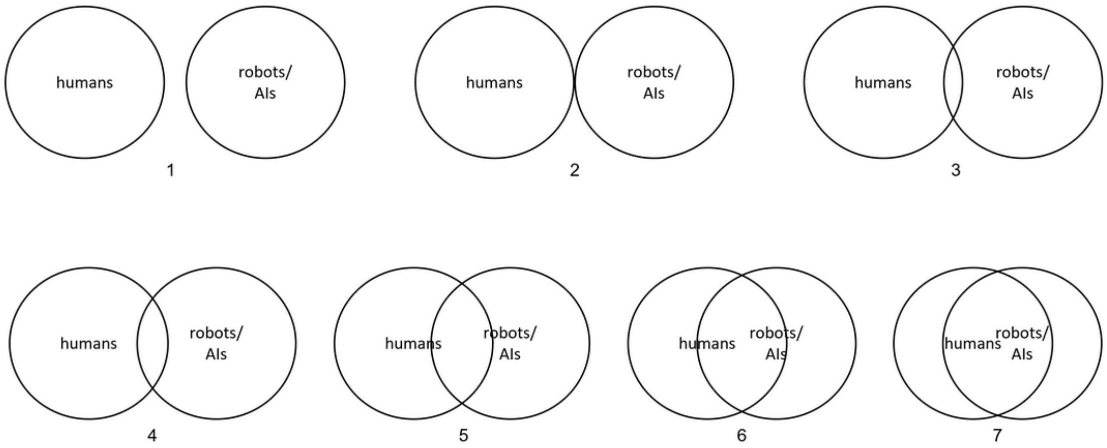


Next

**Which pair of circles best represents how connected machine-like factory production robots are to humans?**

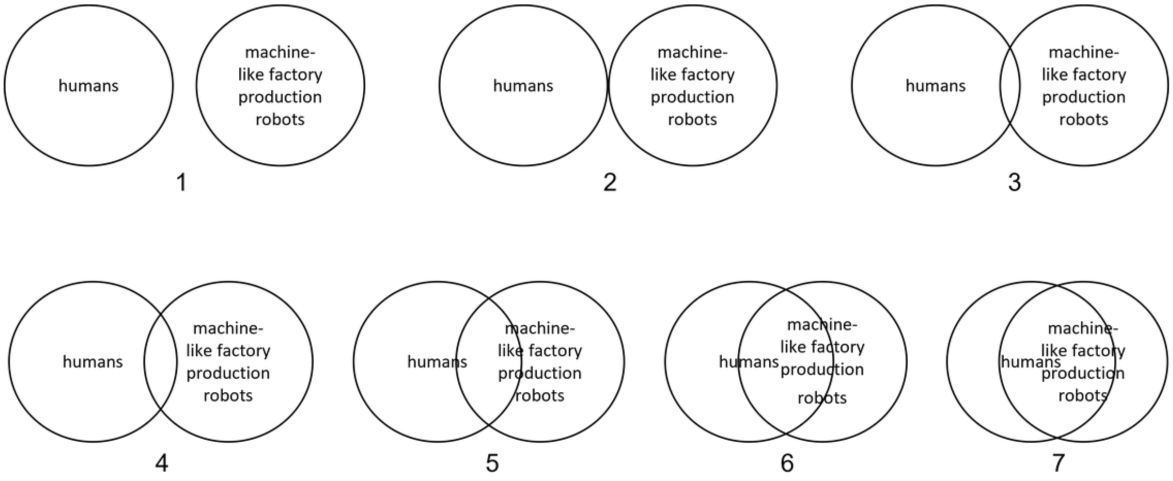


## machine-like factory production robots

who build parts for industry

| |
|---|
| 1 |
| 2 |
| 3 |
| 4 |
| 5 |
| 6 |
| 7 |

Next

**Which pair of circles best represents how connected animal-like companion robots are to humans?**

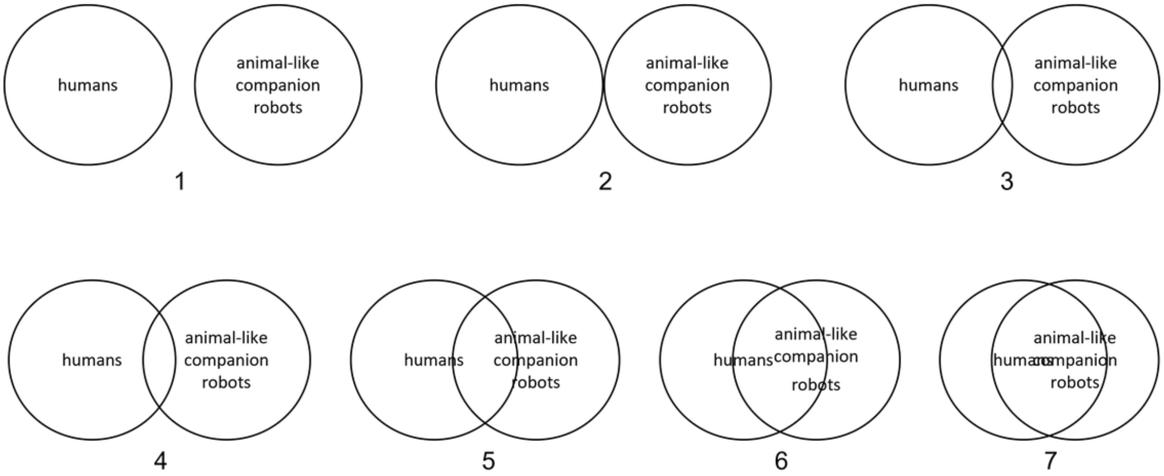


## animal-like companion robots

who socialize with people at home

- 1
- 2
- 3
- 4
- 5
- 6
- 7

Next

**Which pair of circles best represents how connected human-like retail robots are to humans?**

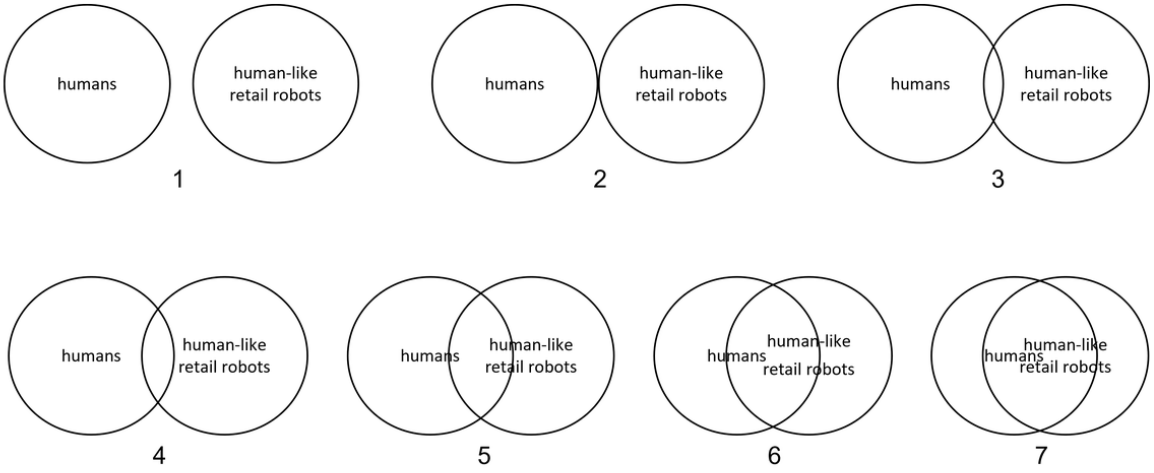


## human-like retail robots

who interact with people at stores and restaurants

- 1
- 2
- 3
- 4
- 5
- 6
- 7

Next

**Which pair of circles best represents how connected machine-like cleaning robots are to humans?**

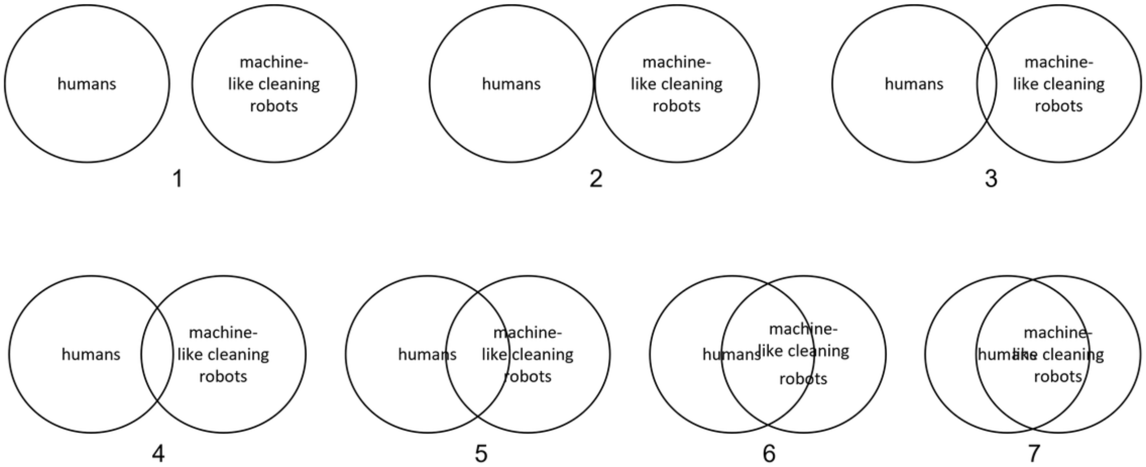


## machine-like cleaning robots

who clean people's spaces

- 1
- 2
- 3
- 4
- 5
- 6
- 7

Next

**Which pair of circles best represents how connected AI personal assistants are to humans?**

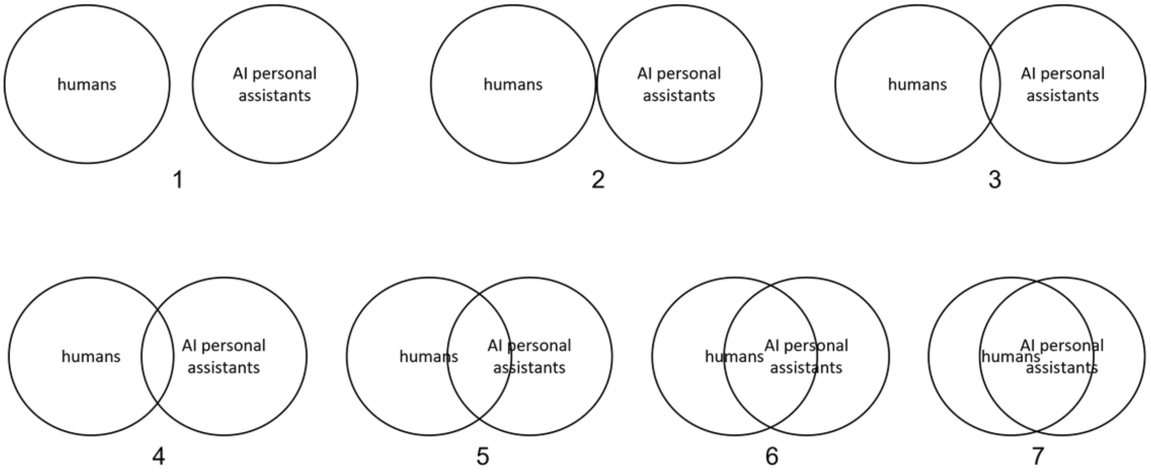


## AI personal assistants

who organize, schedule, and assist people in their daily lives

- 1
- 2
- 3
- 4
- 5
- 6
- 7

Next

**Which pair of circles best represents how connected complex language algorithms are to humans?**

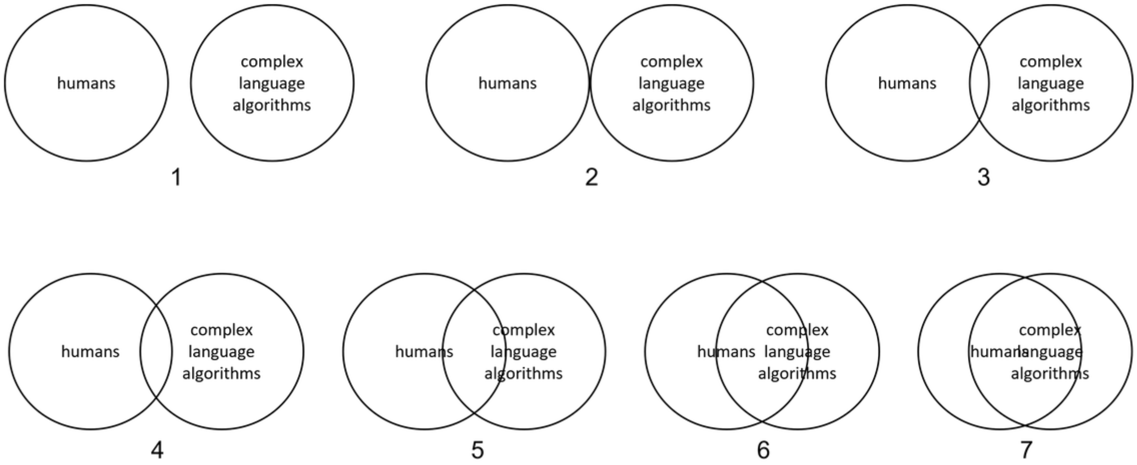


## complex language algorithms

who learn and produce text from data

- 1
- 2
- 3
- 4
- 5
- 6
- 7

Next

**Which pair of circles best represents how connected exact digital copies of human brains are to humans?**

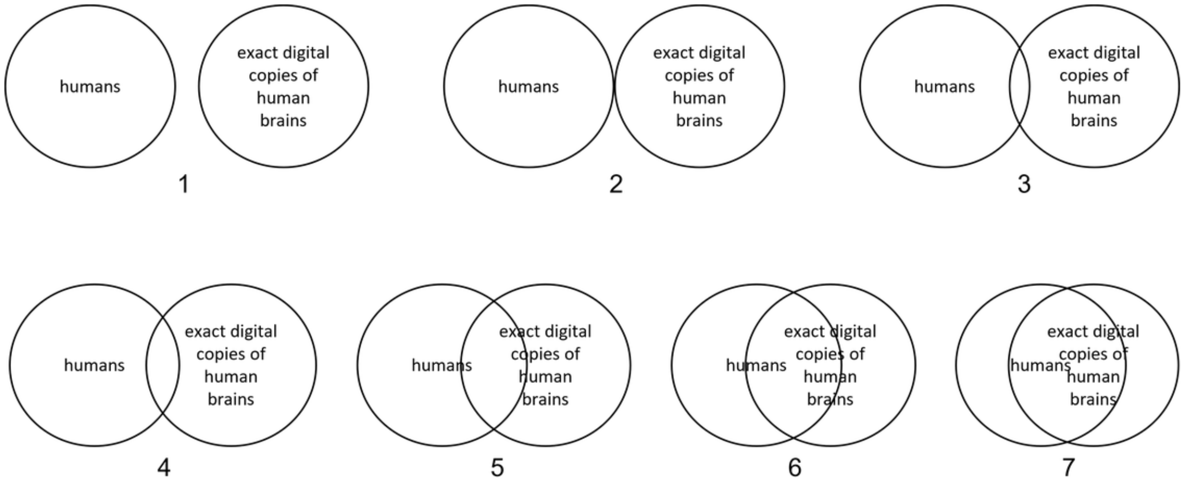


## exact digital copies of human brains

who exist in virtual space

- 1
- 2
- 3
- 4
- 5
- 6
- 7

Next

**Which pair of circles best represents how connected AI video game characters are to humans?**

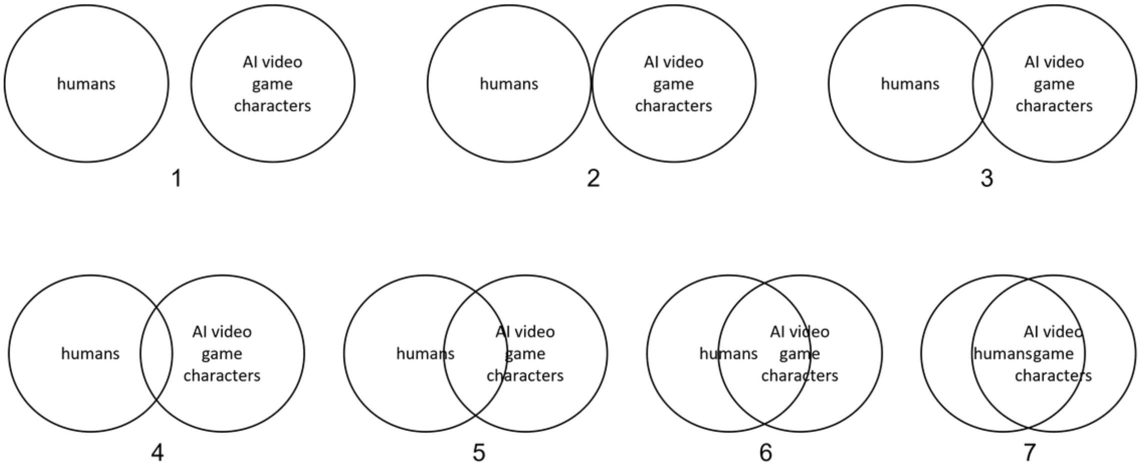


## AI video game characters

who exist only in video games

1

2

3

4

5

6

7

Next

**Which pair of circles best represents how connected exact digital copies of animals are to humans?**

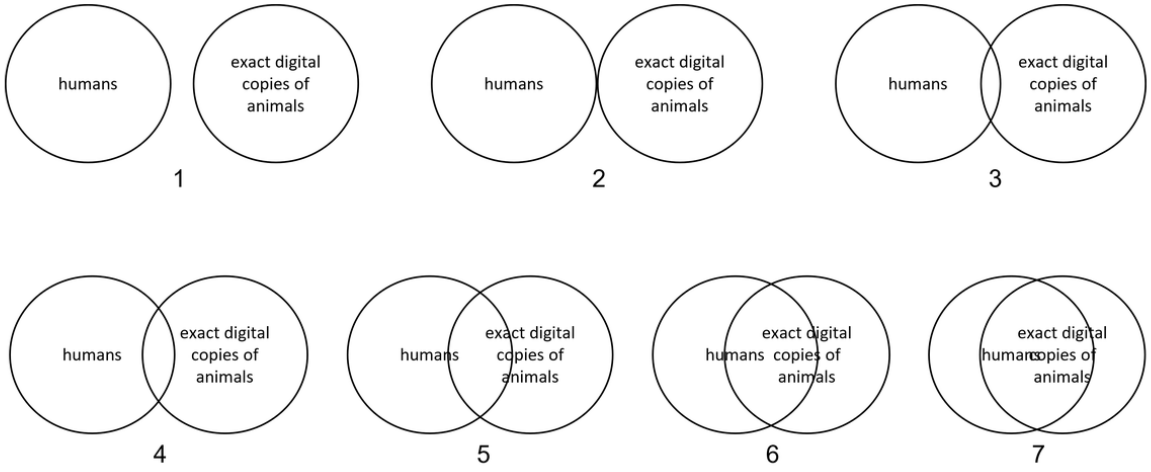


## exact digital copies of animals

who exist in virtual space

| |
|---|
| 1 |
| 2 |
| 3 |
| 4 |
| 5 |
| 6 |
| 7 |

Next

**Which pair of circles best represents how connected virtual avatars are to humans?**

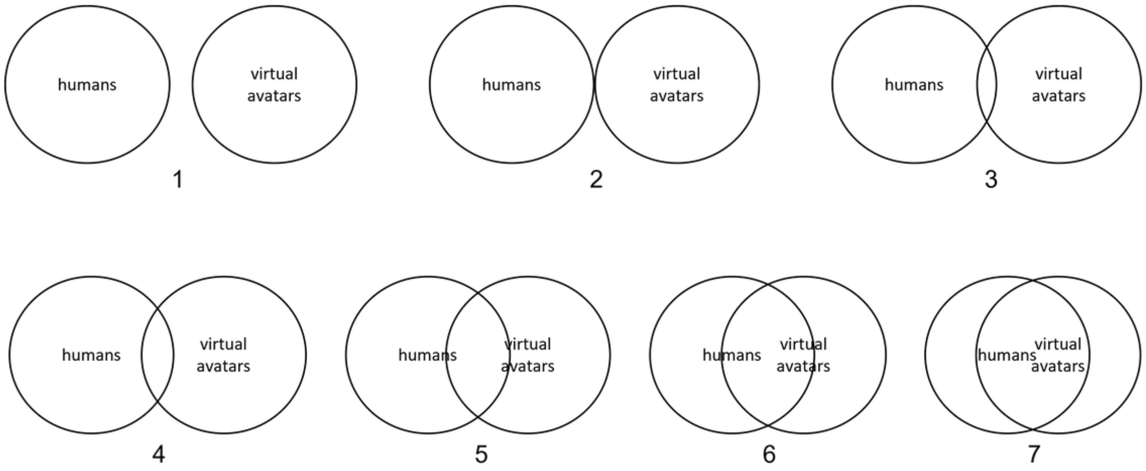


virtual avatars

who exist only in virtual space

| |
|---|
| 1 |
| 2 |
| 3 |
| 4 |
| 5 |
| 6 |
| 7 |

Next

**Which pair of circles best represents how connected human-like companion robots are to humans?**

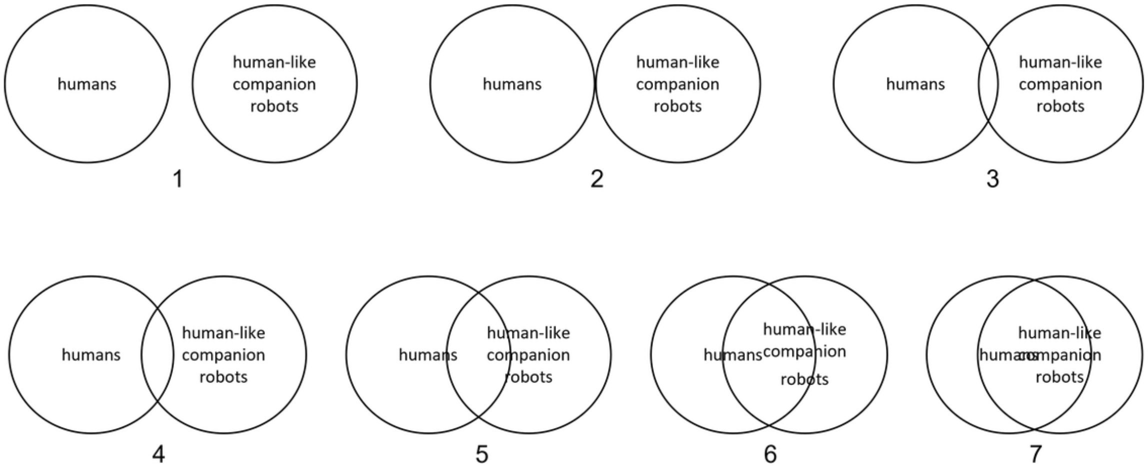


## human-like companion robots

who socialize with people at home

- 1
- 2
- 3
- 4
- 5
- 6
- 7

Next

*Definition Reminder:*

- **Artificial beings** and **robots/AIs** are intelligent entities built by humans, such as robots, virtual copies of human brains, or computer programs that solve problems, with or without a physical body, that may exist now or in the future.
- **Sentience** is the capacity to have positive and negative experiences, such as happiness and suffering.
- **Sentient robots/AIs** are those with the capacity to have positive and negative experiences, such as happiness and suffering.

**To what extent do you agree or disagree with the following statements? (1 = strongly agree, 6 = strongly disagree)**

Robots/AIs should be subservient to humans.

(1) strongly agree

(2) agree

(3) somewhat agree

(4) somewhat disagree

(5) disagree

(6) strongly disagree

No opinion

Robots/AIs may be harmful to people in the USA.

- (1) strongly agree
- (2) agree
- (3) somewhat agree
- (4) somewhat disagree
- (5) disagree
- (6) strongly disagree
- No opinion

Robots/AIs may be harmful to future generations of people.

- (1) strongly agree
- (2) agree
- (3) somewhat agree
- (4) somewhat disagree
- (5) disagree
- (6) strongly disagree
- No opinion

Robots/AIs have been studied systematically since the middle of last century although the word “robot” as we know it first appeared early last century. If you read this, respond with ‘Agree’ for this item.

- (1) strongly agree
- (2) agree
- (3) somewhat agree
- (4) somewhat disagree
- (5) disagree
- (6) strongly disagree
- No opinion

Robots/AIs may be harmful to me personally.

- (1) strongly agree
- (2) agree
- (3) somewhat agree
- (4) somewhat disagree
- (5) disagree
- (6) strongly disagree
- No opinion

Next

*Definition Reminder:*

- **Artificial beings** and **robots/AIs** are intelligent entities built by humans, such as robots, virtual copies of human brains, or computer programs that solve problems, with or without a physical body, that may exist now or in the future.
- **Sentience** is the capacity to have positive and negative experiences, such as happiness and suffering.
- **Sentient robots/AIs** are those with the capacity to have positive and negative experiences, such as happiness and suffering.

Do you think it could ever be possible for robots/AIs to be sentient?

- Yes
- Not sure
- No

Do you think any robots/AIs that currently exist (i.e., those that exist in 2021) are sentient?

- No
- Yes
- Not sure

Next

*Definition Reminder:*

- **Artificial beings** and **robots/AIs** are intelligent entities built by humans, such as robots, virtual copies of human brains, or computer programs that solve problems, with or without a physical body, that may exist now or in the future.
- **Sentience** is the capacity to have positive and negative experiences, such as happiness and suffering.
- **Sentient robots/AIs** are those with the capacity to have positive and negative experiences, such as happiness and suffering.

**If you had to guess, how many years from now do you think that**

robots/AIs will be sentient?

Type a whole number for the number of years. If you think it will never happen, enter 0. If you think it already has happened, enter -1.

the welfare of robots/AIs will be an important social issue?

Type a whole number for the number of years. If you think it will never happen, enter 0. If you think it already has happened, enter -1.

Next

---

*Definition Reminder:*

- **Artificial beings** and **robots/AIs** are intelligent entities built by humans, such as robots, virtual copies of human brains, or computer programs that solve problems, with or without a physical body, that may exist now or in the future.
- **Sentience** is the capacity to have positive and negative experiences, such as happiness and suffering.
- **Sentient robots/AIs** are those with the capacity to have positive and negative experiences, such as happiness and suffering.

How likely is it that robots/AIs will be sentient within the next 100 years?

0%, this definitely will not happen

Slide to answer

100%, this definitely will happen

Next

---

For the questions on the following page, please now imagine a future in which sentient robots/AIs ***have already*** been developed and ***become widespread***. The following questions will ask you about this future world.

Next

*Definition Reminder:*

- **Artificial beings** and **robots/AIs** are intelligent entities built by humans, such as robots, virtual copies of human brains, or computer programs that solve problems, with or without a physical body, that may exist now or in the future.
- **Sentience** is the capacity to have positive and negative experiences, such as happiness and suffering.
- **Sentient robots/AIs** are those with the capacity to have positive and negative experiences, such as happiness and suffering.

**In this future world, to what extent**

are robots/AIs exploited for their labor?

(1) not at all | Slide to answer | (5) very much

are robots/AIs used as subjects in scientific and medical research?

(1) not at all | Slide to answer | (5) very much

is it important to reduce the overall percentage of unhappy sentient robots/AIs?

(1) not at all | Slide to answer | (5) very much

is the welfare of robots/AIs an important social issue?

(1) not at all | Slide to answer | (5) very much

is advocacy for robot/AI rights necessary?

(1) not at all | Slide to answer | (5) very much

are robots/AIs treated cruelly?

(1) not at all | Slide to answer | (5) very much

Next

**Next, you will see some questions that ask about your opinions on some other topics.**

Next

**To what extent do you agree or disagree with the following statements? (1 = strongly agree, 6 = strongly disagree)**

The environment deserves to be included in the moral circle.

- (1) strongly agree
- (2) agree
- (3) somewhat agree
- (4) somewhat disagree
- (5) disagree
- (6) strongly disagree
- No opinion

Animals deserve to be included in the moral circle.

- (1) strongly agree
- (2) agree
- (3) somewhat agree
- (4) somewhat disagree
- (5) disagree
- (6) strongly disagree
- No opinion

The welfare of animals is one of the most important social issues in the world today.

- (1) strongly agree
- (2) agree
- (3) somewhat agree
- (4) somewhat disagree
- (5) disagree
- (6) strongly disagree
- No opinion

The welfare of the environment is one of the most important social issues in the world today.

- (1) strongly agree
- (2) agree
- (3) somewhat agree
- (4) somewhat disagree
- (5) disagree
- (6) strongly disagree
- No opinion

Next

---

*Definition Reminder:*

- **Artificial beings** and **robots/AIs** are intelligent entities built by humans, such as robots, virtual copies of human brains, or computer programs that solve problems, with or without a physical body, that may exist now or in the future.
- **Sentience** is the capacity to have positive and negative experiences, such as happiness and suffering.
- **Sentient robots/AIs** are those with the capacity to have positive and negative experiences, such as happiness and suffering.

**How much do you agree or disagree with the following statements (1 = strongly disagree, 4 = neither agree nor disagree, 7 = strongly agree)?**

Artificial beings contain a spirit.

(1) strongly disagree — Slide to answer — (7) strongly agree

Most people who are important to me think that robots/AIs cannot have feelings.

(1) strongly disagree — Slide to answer — (7) strongly agree

Morally, artificial beings always count for less than humans.

(1) strongly disagree | Slide to answer | (7) strongly agree

The spirits of human, natural, and artificial beings can interact with each other.

(1) strongly disagree | Slide to answer | (7) strongly agree

Humans have the right to use artificial beings however they want to.

(1) strongly disagree | Slide to answer | (7) strongly agree

Next

---

*Definition Reminder:*

- **Artificial beings** and **robots/AIs** are intelligent entities built by humans, such as robots, virtual copies of human brains, or computer programs that solve problems, with or without a physical body, that may exist now or in the future.
- **Sentience** is the capacity to have positive and negative experiences, such as happiness and suffering.
- **Sentient robots/AIs** are those with the capacity to have positive and negative experiences, such as happiness and suffering.

**Please answer the following questions (0 = not at all, 10 = very much).**

To what extent does the average computer have a mind of its own?

(0) not at all | Slide to answer | (10) very much

To what extent does the average AI have intentions?

(0) not at all | Slide to answer | (10) very much

To what extent does the average digital simulation have emotions?

(0) not at all | Slide to answer | (10) very much

To what extent does the average robot have consciousness?

(0) not at all | Slide to answer | (10) very much

Next

---

**Next, you will see questions about your own experience with robots/AIs.**

Next

---

## AIs at home

Do you own AI or robotic devices that can detect their environment and respond appropriately? For example, you might own...

- a home assistant that can detect whatever you say and respond in kind
- a home assistant that can control the temperature and ambient lighting based on feedback it receives from the environment
- a robotic vacuum cleaner that decides where to move by itself
- a self-driving car that monitors its environment and drives itself
- a companion robot that can interact with you socially

Do you own AI or robotic devices that can detect their environment and respond appropriately?

- No
- Yes

Next

## AIs at work

Do you work with AI or robotic devices at your job? For example, you might work with a robot/AI...

- for research or scientific purposes
- for information or fact checking
- for facial recognition
- for healthcare diagnoses
- for making social work or legal decisions
- for aerial photography or mapping
- for disaster response
- for industrial production
- for creative arts

### Do you work with AI or robotic devices at your job?

No

Yes

Next

## Smart devices

Do you own a smart device that has some ability to detect its environment and network with other devices but that cannot respond to everything you might say or that requires you to pre-program its routines? For instance, you might own...

- a smartphone
- a smart TV
- smart speakers
- a smart coffee maker
- a smart toaster
- smart light bulbs

Do you own a smart device that has some ability to detect its environment and network with other devices but that cannot respond to everything you might say or that requires you to pre-program its routines?

- Yes
- No

Next

Have you ever experienced any of the following? (check all that apply)

- Saw a robot being physically abused or attacked by humans ☐
- Saw a video, gif, or other media of a robot being physically abused or attacked by humans ☐
- Had a conversation with a robot/AI ☐
- Read a book or article that discussed AI ethics or moral status ☐
- Had a conversation with a family member or friend about robots/AIs ☐
- None of the above ☐

Next

How often do you interact with AI or robotic devices that respond to you and that can choose their own behavior?

- (0) Never or Not applicable
- (1) Only on rare occasions
- (2) A few times a year
- (3) Monthly
- (4) Weekly
- (5) Daily

How often do you read or watch robot/AI-related stories, movies, TV shows, comics, news, product descriptions, conference papers, journal papers, blogs, or other material?

- (0) Never or Not applicable
- (1) Only on rare occasions
- (2) A few times a year
- (3) Monthly
- (4) Weekly
- (5) Daily

Next

How would you describe your political views?

1 = very liberal, 3 = moderate, 5 = very conservative

(1) very liberal | Slide to answer | (5) very conservative

What is your present religion, if any?

- Buddhist
- Christian-Catholic (for example Roman Catholic and Orthodox)
- Christian-Protestant (for example Episcopalian, Presbyterian, United Church of Christ, Methodist, Baptist, Lutheran)
- Hindu
- Jain
- Jewish
- Muslim
- Shinto
- Sikh
- Atheist (do not believe in God)
- Agnostic (not sure if there is a God)
- No religion
- Something else (if you answered 'something else' for religion, please specify).
- Prefer not to say

If you answered 'something else' for religion, please specify.

Which of these best describes what you currently eat?

- Meat-eater (no restrictions on animal products)
- Pescatarian (no chicken, beef, or any meats other than fish)
- Vegetarian (no meat)
- Vegan (no animal products)
- Other restrictions on animal products

Next

Thank you for your participation. If you have any feedback or additional comments, please leave them here and press 'Submit' to finish the survey.

Submit
