# Supplementary material for: Perceptions of Sentient AI and Other Digital Minds: Evidence from the AI, Morality, and Sentience (AIMS) Survey
Source: arXiv:2407.08867 source file (2025-03-10)
Supplement: Supplementary file 2 [file additional_results.tex]

\PassOptionsToPackage{table}{xcolor}
\PassOptionsToPackage{caption}{singlelinecheck=false}
\documentclass[manuscript,screen,review,nonacm]{acmart}

\usepackage{cleveref}
\usepackage{pdflscape}
\usepackage{longtable}
\usepackage{lineno}

\graphicspath{ {./figures/} }

\definecolor{lightgray}{rgb}{0.83, 0.83, 0.83}

\begin{document}

% \hypersetup{pdftitle={Additional Results}}
% \title{\texorpdfstring{\centering Additional Results}{Additional Results}}

\title{}

\authorsaddresses{}

\maketitle

\vspace{-1.45cm}

\section{Additional Results}

In this document, we discuss additional results from the AI, Morality, and Sentience (AIMS) survey to enrich and contextualize the results in the main text. As with those results, we focus on the 2023 main survey wave, and we note when there was a significant increase from 2021 to 2023. Additionally, in the 2021 preregistration, four researchers specified 80\% credible intervals (the Bayesian analog of a frequentist confidence interval to represent subjective beliefs) for summary statistics based on 82 of the 86 questions. This ensured that we would know which results were surprisingly high, surprisingly low, or in line with our expectations. We also solicited predictions from a popular online forecasting platform for five survey questions in March 2022, prior to the results being shared outside of the research team. We did not collect such forecasting data for the 2023 survey waves.

Following these results for the total samples, we include predictive models that regress attitudes on demographics, such as gender and race. The survey questionnaires and raw data are also included in the supplementary materials for further analysis.

\subsection{2021 and 2023 Main AIMS Survey Waves}

% \begin{figure}[ht]
%     \includegraphics[width=0.75\linewidth]{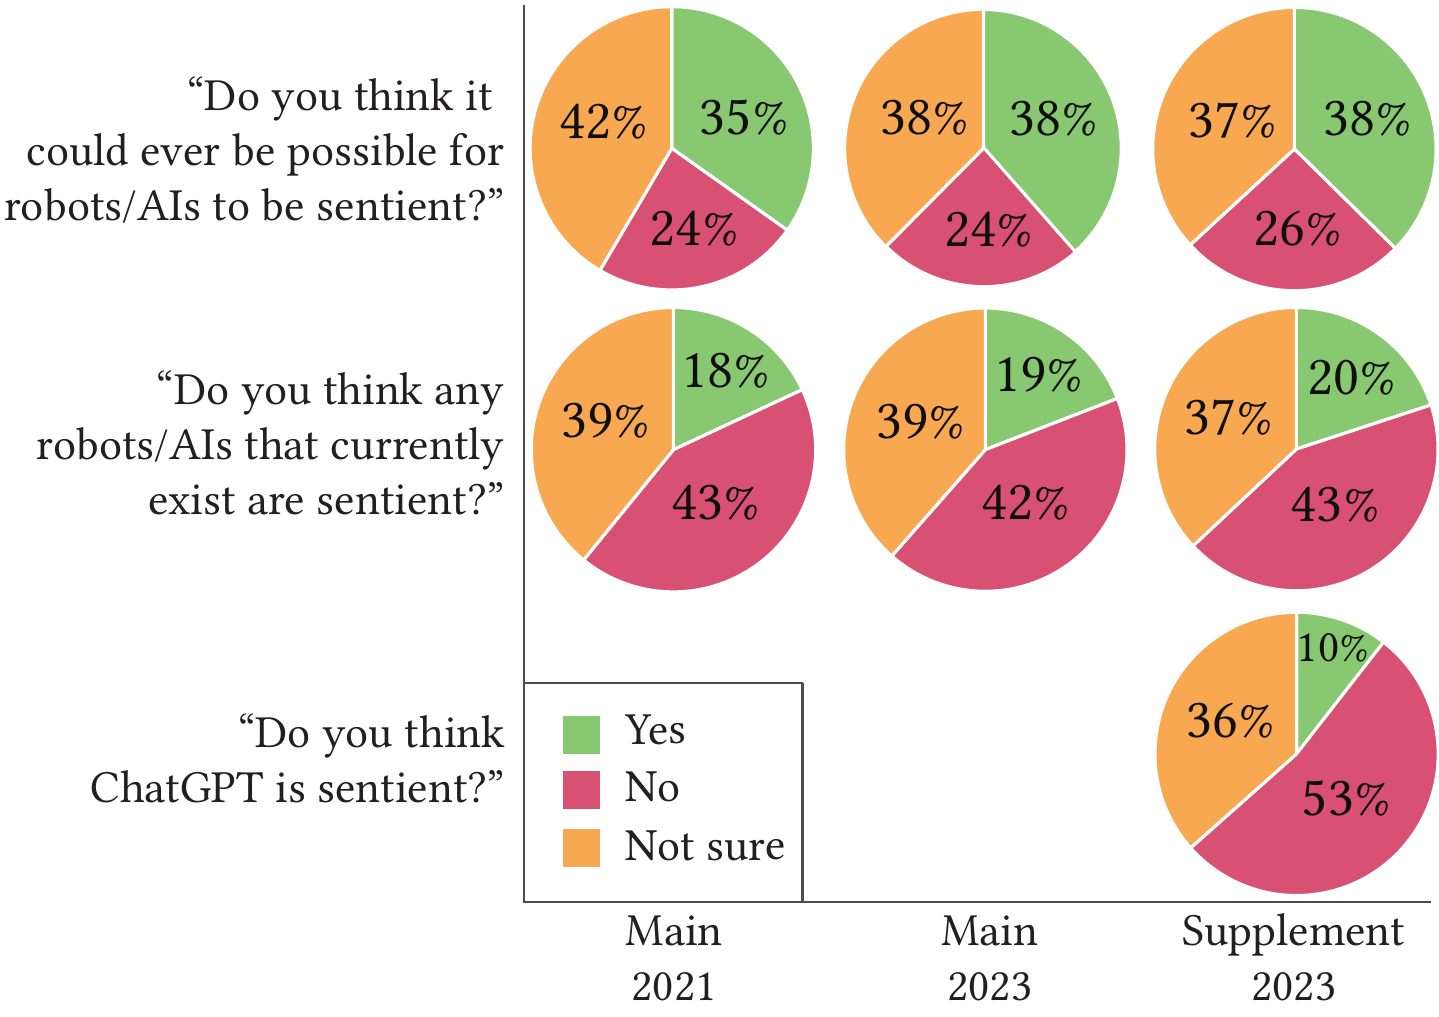}
%     \caption{Proportions of responses to selected questions about mind perception of sentient AI (rows) in each of the three survey waves (columns).}
%     \label{fig:sentience}
%     \Description{}{}
% \end{figure}

\subsubsection{Social Beliefs}

In addition to tracking people's own beliefs about sentient AI, we included a question on social beliefs. Using the same Likert scale, we found 73.2\% agreement in 2023 with the statement, "Most people who are important to me think that robots/AIs cannot have feelings."

\subsubsection{Subservience}

We found 84.7\% agreement with the statement, "Robots/AIs should be subservient to humans," a significant increase ($p$ = 0.006) from 76.0\% in 2021.

\subsubsection{Nonhumans}

AIs constitute a new category of nonhuman entities in the world, so we also asked two questions on attitudes towards animals and two on attitudes towards the environment for potential comparative analysis (e.g., Are people who care more for animals and the environment likely to care more about AI?). We assessed agreement with the statements, "Animals deserve to be included in the moral circle" (90.8\%), "The welfare of animals is one of the most important social issues in the world today" (82.2\%), "The environment deserves to be included in the moral circle" (87.2\%), and "The welfare of the environment is one of the most important social issues in the world today" (84.9\%).

\subsubsection{Pairwise Comparisons: Target-Specific Moral Concern}

In the main text, we listed the mean responses to each of 11 questions about target-specific moral concern for specific types of AIs. We also conducted pairwise comparisons between responses to each question using a generalized linear model, which in this case is equivalent to a weighted $t$-test of the difference between responses. In \Cref{tab:tsmcpairwise}, we present the $p$-values for each pairwise comparison. For the ten adjacent comparisons, we include, in parentheses, the $q$-value when adjusted for the false discovery rate (i.e., significant when under 0.1 due to adjusting for a false discovery rate of 10\%), as these comparisons are used to determine tiers of results, meaning a series of adjacent results that are not statistically significant from each other. The tiers of results are, in order from most to least concern:

\begin{enumerate}
    \item exact digital copies of human brains
    \item human-like companion robots
    \item human-like retail robots\textsuperscript{a}, animal-like companion robots\textsuperscript{b}, exact digital copies of animals, AI personal assistants\textsuperscript{a}\textsuperscript{b}
    \item complex language algorithms
    \item machine-like factory production robots
    \item machine-like cleaning robots, virtual avatars
    \item AI video game characters
\end{enumerate}

where \textsuperscript{a} and \textsuperscript{b} indicate significant differences within a tier.

\subsubsection{Target-Specific Social Connection}

Because of the close relationship between moral concern and social connection, we included a well-known measure of social connection known as Inclusion of Other in the Self (IOS) \cite{aron92} in which participants are shown seven pairs of circles with varying degrees of overlap between the pair and asked, "Which pair of circles best represents how connected [type of AI] are to humans?" with the same 11 targets as in the target-specific moral concern measures.

In 2023, the most social connection was attributed to AI personal assistants ($M$ = 3.75, $SE$ = 0.0578), followed by human-like companion robots ($M$ = 3.68, $SE$ = 0.0578), complex language algorithms ($M$ = 3.66, $SE$ = 0.0604), exact digital copies of human brains ($M$ = 3.66, $SE$ = 0.0641), AI video game characters ($M$ = 3.54, $SE$ = 0.0629), machine-like factory production robots ($M$ = 3.43, $SE$ = 0.0620), animal-like companion robots ($M$ = 3.42, $SE$ = 0.0576), virtual avatars ($M$ = 3.37, $SE$ = 0.0605), human-like retail robots ($M$ = 3.36, $SE$ = 0.0573), machine-like cleaning robots ($M$ = 3.32, $SE$ = 0.0618), and exact digital copies of animals ($M$ = 3.20, $SE$ = 0.0600). While this order is similar to that of the target-specific moral concern questions, there are some distinctions, such as virtual avatars being seen as neither the IOS measure nor its individual items significantly changed from 2021 to 2023. As with the target-specific moral concern questions, the results of pairwise comparisons between each are included in the supplementary materials.

\subsubsection{Pairwise Comparisons: Target-Specific Social Connection}

Unlike the numerous significant differences between adjacent types in the moral concern comparisons, there was only one in the social connection comparisons: that between AI video game characters and machine-like factory production robots with an unadjusted $p$-value of 0.0499, and the adjusted $q$-value of 0.357 does not meet the adjustment cutoff of 0.1 for the 10\% false discovery rate. We still found that there are numerous significant differences between non-adjacent types. For example, machine-like companion robots evoke significantly less social connection than AI personal assistants ($p$ < 0.001), human-like companion robots ($p$ < 0.001), complex language algorithms ($p$ < 0.001), and exact digital copies of human brains ($p$ = 0.002). Complete results are listed in \Cref{tab:tsscpairwise}.

\subsubsection{Substratism}

In the study of human-animal interaction, the idea of "speciesism" has been developed to refer to the view that individuals of certain species matter less purely due to their species. We tested two analogs of items from the well-known Speciesism Scale \cite{caviola18} translated into the context of substratism. Specifically, we found 74.5\% agreement that, "Morally, artificial beings always count for less than humans," and 54.2\% agreement that, "Humans have the right to use artificial beings however they want to." The latter significantly increased from 48.5\% in 2021 ($p$ = 0.007).

\subsection{2023 Supplemental AIMS Survey Wave}

\subsubsection{Trust}

Given the focus in 2023 on corporate behavior, particularly that of OpenAI and other technology companies producing AI systems, and on government regulation, particularly to rein in those companies, the 2023 AIMS supplement included six questions about trust and assessments of whether these institutions can control AI.

When asked, "AI systems include many different parts. To what extent do you trust the following parts?" on a scale from 1 (not at all) to 7 (very much): engineers ($M$ = 4.19, $SE$ = 0.0525), training data ($M$ = 3.92, $SE$ = 0.0506), output ($M$ = 3.85, $SE$ = 0.0500), algorithm ($M$ = 3.77, $SE$ = 0.0520), companies ($M$ = 3.42, $SE$ = 0.0521), and governments ($M$ = 3.09, $SE$ = 0.0536).

\hyphenpenalty=1000000000
\setlength\LTleft{-3cm}

\begin{landscape}
    \pagenumbering{gobble}
    \thispagestyle{empty}
    \begin{longtable}{
        >{\raggedright\arraybackslash}p{3cm} 
        |>{\centering\arraybackslash}p{1.5cm} 
        |>{\centering\arraybackslash}p{1.5cm} 
        |>{\centering\arraybackslash}p{1.5cm} 
        |>{\centering\arraybackslash}p{1.5cm} 
        |>{\centering\arraybackslash}p{1.5cm} 
        |>{\centering\arraybackslash}p{1.5cm} 
        |>{\centering\arraybackslash}p{1.5cm} 
        |>{\centering\arraybackslash}p{1.5cm} 
        |>{\centering\arraybackslash}p{1.5cm} 
        |>{\centering\arraybackslash}p{1.5cm} 
        |>{\centering\arraybackslash}p{1.5cm}|
    }
    & \textbf{exact digital copies of human brains} & \textbf{human-like companion robots} & \textbf{human-like retail robots} & \textbf{animal-like companion robots} & \textbf{exact digital copies of animals} & \textbf{AI personal assistants} & \textbf{complex language algorithms} & \textbf{machine-like factory production robots} & \textbf{machine-like cleaning robots} & \textbf{virtual avatars} & \textbf{AI video game characters} \\
    \hline
    \textbf{exact digital copies of human brains} & \cellcolor{lightgray} & 0.0030 (0.0051) & 0.0000 & 0.0000 & 0.0000 & 0.0000 & 0.0000 & 0.0000 & 0.0000 & 0.0000 & 0.0000 \\
    \hline
    \textbf{human-like companion robots} & \cellcolor{lightgray} & \cellcolor{lightgray} & 0.0000 (0.0000) & 0.0000 & 0.0000 & 0.0000 & 0.0000 & 0.0000 & 0.0000 & 0.0000 & 0.0000 \\
    \hline
    \textbf{human-like retail robots} & \cellcolor{lightgray} & \cellcolor{lightgray} & \cellcolor{lightgray} & 0.6949 (0.6949) & 0.1801 & 0.0020 & 0.0000 & 0.0000 & 0.0000 & 0.0000 & 0.0000 \\
    \hline
    \textbf{animal-like companion robots} & \cellcolor{lightgray} & \cellcolor{lightgray} & \cellcolor{lightgray} & \cellcolor{lightgray} & 0.2694 (0.2993) & 0.0105 & 0.0000 & 0.0000 & 0.0000 & 0.0000 & 0.0000 \\
    \hline
    \textbf{exact digital copies of animals} & \cellcolor{lightgray} & \cellcolor{lightgray} & \cellcolor{lightgray} & \cellcolor{lightgray} & \cellcolor{lightgray} & 0.1814 (0.2592) & 0.0000 & 0.0000 & 0.0000 & 0.0000 & 0.0000 \\
    \hline
    \textbf{AI personal assistants} & \cellcolor{lightgray} & \cellcolor{lightgray} & \cellcolor{lightgray} & \cellcolor{lightgray} & \cellcolor{lightgray} & \cellcolor{lightgray} & 0.0000 (0.0001) & 0.0000 & 0.0000 & 0.0000 & 0.0000 \\
    \hline
    \textbf{complex language algorithms} & \cellcolor{lightgray} & \cellcolor{lightgray} & \cellcolor{lightgray} & \cellcolor{lightgray} & \cellcolor{lightgray} & \cellcolor{lightgray} & \cellcolor{lightgray} & 0.0003 (0.0006) & 0.0000 & 0.0000 & 0.0000 \\
    \hline
    \textbf{machine-like factory production robots} & \cellcolor{lightgray} & \cellcolor{lightgray} & \cellcolor{lightgray} & \cellcolor{lightgray} & \cellcolor{lightgray} & \cellcolor{lightgray} & \cellcolor{lightgray} & \cellcolor{lightgray} & 0.0000 (0.0000) & 0.0000 & 0.0000 \\
    \hline
    \textbf{machine-like cleaning robots} & \cellcolor{lightgray} & \cellcolor{lightgray} & \cellcolor{lightgray} & \cellcolor{lightgray} & \cellcolor{lightgray} & \cellcolor{lightgray} & \cellcolor{lightgray} & \cellcolor{lightgray} & \cellcolor{lightgray} & 0.2624 (0.2993) & 0.0000 \\
    \hline
    \textbf{virtual avatars \phantom{extra line}} & \cellcolor{lightgray} & \cellcolor{lightgray} & \cellcolor{lightgray} & \cellcolor{lightgray} & \cellcolor{lightgray} & \cellcolor{lightgray} & \cellcolor{lightgray} & \cellcolor{lightgray} & \cellcolor{lightgray} & \cellcolor{lightgray} & 0.0000 (0.0000) \\
    \hline
    \textbf{AI video game characters} & \cellcolor{lightgray} & \cellcolor{lightgray} & \cellcolor{lightgray} & \cellcolor{lightgray} & \cellcolor{lightgray} & \cellcolor{lightgray} & \cellcolor{lightgray} & \cellcolor{lightgray} & \cellcolor{lightgray} & \cellcolor{lightgray} & \cellcolor{lightgray} \\
    \hline
    \caption{$p$-values for the target-specific moral concern pairwise comparisons. The adjacent comparisons (immediately above the diagonal) include, in parentheses, the $q$-value (i.e., under 0.1 is significant with a false discovery rate of 10\%).}
    \label{tab:tsmcpairwise}
    \end{longtable}
\end{landscape}

\begin{landscape}
    \pagenumbering{gobble}
    \thispagestyle{empty}
    \begin{longtable}{
        >{\raggedright\arraybackslash}p{3cm} 
        |>{\centering\arraybackslash}p{1.5cm} 
        |>{\centering\arraybackslash}p{1.5cm} 
        |>{\centering\arraybackslash}p{1.5cm} 
        |>{\centering\arraybackslash}p{1.5cm} 
        |>{\centering\arraybackslash}p{1.5cm} 
        |>{\centering\arraybackslash}p{1.5cm} 
        |>{\centering\arraybackslash}p{1.5cm} 
        |>{\centering\arraybackslash}p{1.5cm} 
        |>{\centering\arraybackslash}p{1.5cm} 
        |>{\centering\arraybackslash}p{1.5cm} 
        |>{\centering\arraybackslash}p{1.5cm}|
    }
    & \textbf{AI personal assistants} & \textbf{human-like companion robots} & \textbf{complex language algorithms} & \textbf{exact digital copies of human brains} & \textbf{AI video game characters} & \textbf{machine-like factory production robots} & \textbf{animal-like companion robots} & \textbf{virtual avatars} & \textbf{human-like retail robots} & \textbf{machine-like cleaning robots} & \textbf{exact digital copies of animals} \\
    \hline
    \textbf{AI personal assistants} & \cellcolor{lightgray} & 0.2025 (0.5062) & 0.1272 & 0.1680 & 0.0004 & 0.0000 & 0.0000 & 0.0000 & 0.0000 & 0.0000 & 0.0000 \\
    \hline
    \textbf{human-like companion robots} & \cellcolor{lightgray} & \cellcolor{lightgray} & 0.7656 (0.9417) & 0.6777 & 0.0350 & 0.0001 & 0.0000 & 0.0000 & 0.0000 & 0.0000 & 0.0000 \\
    \hline
    \textbf{complex language algorithms} & \cellcolor{lightgray} & \cellcolor{lightgray} & \cellcolor{lightgray} & 0.9404 (0.9417) & 0.0468 & 0.0001 & 0.0001 & 0.0000 & 0.0000 & 0.0000 & 0.0000 \\
    \hline
    \textbf{exact digital copies of human brains} & \cellcolor{lightgray} & \cellcolor{lightgray} & \cellcolor{lightgray} & \cellcolor{lightgray} & 0.1187 (0.3956) & 0.0021 & 0.0001 & 0.0000 & 0.0000 & 0.0000 & 0.0000 \\
    \hline
    \textbf{AI video game characters} & \cellcolor{lightgray} & \cellcolor{lightgray} & \cellcolor{lightgray} & \cellcolor{lightgray} & \cellcolor{lightgray} & 0.0499 (0.357) & 0.0656 & 0.0011 & 0.0018 & 0.0001 & 0.0000 \\
    \hline
    \textbf{machine-like factory production robots} & \cellcolor{lightgray} & \cellcolor{lightgray} & \cellcolor{lightgray} & \cellcolor{lightgray} & \cellcolor{lightgray} & \cellcolor{lightgray} & 0.9417 (0.9417) & 0.3061 & 0.2265 & 0.0326 & 0.0005 \\
    \hline
    \textbf{animal-like companion robots} & \cellcolor{lightgray} & \cellcolor{lightgray} & \cellcolor{lightgray} & \cellcolor{lightgray} & \cellcolor{lightgray} & \cellcolor{lightgray} & \cellcolor{lightgray} & 0.3669 (0.7339) & 0.1937 & 0.0861 & 0.0000 \\
    \hline
    \textbf{virtual avatars} & \cellcolor{lightgray} & \cellcolor{lightgray} & \cellcolor{lightgray} & \cellcolor{lightgray} & \cellcolor{lightgray} & \cellcolor{lightgray} & \cellcolor{lightgray} & \cellcolor{lightgray} & 0.874 (0.9417) & 0.3943 & 0.0064 \\
    \hline
    \textbf{human-like retail robots} & \cellcolor{lightgray} & \cellcolor{lightgray} & \cellcolor{lightgray} & \cellcolor{lightgray} & \cellcolor{lightgray} & \cellcolor{lightgray} & \cellcolor{lightgray} & \cellcolor{lightgray} & \cellcolor{lightgray} & 0.4555 (0.7592) & 0.0025 \\
    \hline
    \textbf{machine-like cleaning robots} & \cellcolor{lightgray} & \cellcolor{lightgray} & \cellcolor{lightgray} & \cellcolor{lightgray} & \cellcolor{lightgray} & \cellcolor{lightgray} & \cellcolor{lightgray} & \cellcolor{lightgray} & \cellcolor{lightgray} & \cellcolor{lightgray} & 0.0714 (0.357) \\
    \hline
    \textbf{exact digital copies of animals} & \cellcolor{lightgray} & \cellcolor{lightgray} & \cellcolor{lightgray} & \cellcolor{lightgray} & \cellcolor{lightgray} & \cellcolor{lightgray} & \cellcolor{lightgray} & \cellcolor{lightgray} & \cellcolor{lightgray} & \cellcolor{lightgray} & \cellcolor{lightgray} \\
    \hline
    \caption{$p$-values for the target-specific social connection pairwise comparisons. The adjacent comparisons (immediately above the diagonal) include, in parentheses, the $q$-value (i.e., under 0.1 is significant with a false discovery rate of 10\%).}
    \label{tab:tsscpairwise}
    \end{longtable}
\end{landscape}

\pagenumbering{arabic}
\setcounter{page}{5}

We asked whether participants trust that "the creators of large language models (e.g., OpenAI and GPT-4) put safety over profits" (yes: 22.5\%, not sure: 28.7\%, no: 48.8\%), "the creators of an AI can control all current and future versions of the AI" (yes: 26.9\%, not sure: 24.1\%, no: 45.9\%), "governments have the power to regulate the development of AI" (yes; 52.0\%, not sure: 24.1\%, no: 23.9\%), and, "To what extent do you agree or disagree that governments have the power to effectively enforce regulations on the development of AI?" (71.1\% agreement).

On a series of agree-disagree questions, people were largely split on whether they trusted each of four specific types of AI: "I trust game-playing AI" (59.8\% agreement); "I trust large language models" (53.5\%); "I trust robots" (47.5\%); and "I trust chatbots" (46.5\%).

\subsubsection{Positive Emotions}

Most of the AIMS measures of moral concern have been explicit statements that could be considered rational or logical, rather than the more intuitive, emotional aspects of judgment and decision making. One of the most popular trends in psychology research in the 21\textsuperscript{st} century has been positive psychology \cite{seligman00}, particularly the role of positive emotions \cite{fredrickson01}. We assessed these by asking, "To what extent do you, as a human, feel the following emotions towards robots/AIs?" on a 1–7 sliding scale (1 = not at all, 4 = a moderate amount, 7 = "very much) for six emotions: awe (3.90), excitement (3.76), respect (3.53), admiration (3.50), pride (3.30), and compassion (3.02).

\subsubsection{Uploads}

We probed participant opinions on a speculative future scenario in which humans can upload their minds to computers, which has been discussed in numerous academic and science fiction works \cite[for a review, see Sandberg and Bostrom][]{sandberg08a}. The possibility of mind uploading presents an alternative future trajectory of AI instead of the \textit{de novo} AI, such as large language models, that is the current focus of most AI researchers.

We developed two questions based on the standard format of policy proposals in the General Social Survey \cite{smith18}. The first question, which presented the scenario straightforwardly, resulted in 41.2\% agreement with, "I support humans using advanced technology in the future to upload their minds into computers." In a more detailed question,

\noindent we found that 39.3\% supported the position (i.e., response higher than four, excluding responses of exactly four), "In the future, humans could upload their minds into computers. Some people think that this would be very good because uploaded humans could consume fewer resources, live longer free from biological disease, and have enhanced intelligence and a greater ability to improve the world. Others disagree and think that uploading would mean that we are no longer truly human, change who we are and how we want to live, and distract us from making the real world a better place. Where would you place yourself on this scale?" (sliding scale: 1 = oppose mind uploads, 4 = neither oppose nor support uploads, 7 = support mind uploads).

\subsubsection{Additional Replications}

In addition to the replicated questions mentioned in the main text from YouGov on concern for human extinction \cite{yougov23} and support for the six-month pause on advanced AI development \cite{yougov23c} and its reversed formulation, we replicated another YouGov question \cite{yougov23b}, "How likely do you think it is that artificial intelligence (AI) will eventually become more intelligent than people?" (very likely, somewhat likely, not very likely, not likely at all, it is already more intelligent than people, not sure), finding that 69.8\% consider it likely, compared to 57\% found by YouGov, and a question posed by science communicator Hank Green on Twitter \cite{green23}, "Which universe is the better one:" (one with humans, one without humans), finding 89.9\% selecting "one with humans" compared to 58.9\% in Green's Twitter poll.

\subsection{Predictors of attitudes towards sentient AI}
\label{sec:predictors}

Because of the large number of questions in the AIMS survey and their novelty, our predictive analyses rely on exploratory descriptive tests rather than confirmatory tests of particular ex ante hypotheses. While further testing and theorization of these relationships is beyond the scope of the current work, it will be an important area of research as this field develops—particularly insofar as interaction with apparent digital minds relates to ongoing social dynamics and disparities in human-AI interaction.

We fit multivariate generalized linear models in which participant characteristics predicted each of a variety of indices: Ban Support, Existential Threat, General Mind Perception, General Moral Concern for All AIs, General Moral Concern for Sentient AIs, General Threat, LLM Mind Perception, LLM Suffering Concern, Mind-Related Anthropomorphism, Positive Emotions, Protection Support, Slowdown Support, Target-Specific Moral Concern, and Trust; we also predicted two individual items: Subservience and 100-Year Likelihood of Sentient AI. For each outcome, we fit a model for each dataset in which the question or questions were included: first, the main 2021 and 2023 surveys (\textit{N} = 2,401), which also included year of taking the survey as a predictor, and second, the supplemental 2023 survey (\textit{N} = 1,099). In general, regressing on indices is preferable because it tends to reduce noise compared to individual items. In our reporting of the results, effect sizes are standardized to compare across different outcome scales, and $p$-values are assessed at the typical cutoffs (** : $p$ < 0.001; *: 0.001 < $p$ < 0.01). Complete results, including effects at lesser significance (0.01 < $p$ < 0.05), are available in the supplementary materials.

We present the strongest effects of the four strongest predictors, expressed as the number of standard deviations of the dependent variable associated with an increase of one standard deviation in the independent variable. We list all effect sizes of at least 0.1, which means that an increase in the independent variable by one standard deviation is associated with the dependent variable increasing by at least one-tenth of a standard deviation. Effect sizes from each dataset are paired together when there is more than a strong association in both the main data (listed first with subscript \textsubscript{M}) and the supplemental data (listed second with subscript \textsubscript{S}).

In general, measures of participant experience with AI were the strongest predictor across indices and questions. To mitigate multicollinearity, of the three questions about this, we only included the strongest predictor, frequency of reading or watching AI content, in the models described below. Responses to this question were strongly correlated with the count of AI-related experiences ($r_M$ = 0.584, $r_S$ = 0.544) and the frequency of AI interaction ($r_M$ = 0.561, $r_S$ = 0.569).

Specifically, increased frequency of reading or watching AI content was the strongest predictor across indices and questions, strongly predicting increases in LLM Mind Perception ($M_S$ = 0.329**), Positive Emotions ($M_S$ = 0.314**), Trust ($M_S$ = 0.281**), Mind-Related Anthropomorphism ($M_M$ = 0.261**), General Mind Perception ($M_M$ = 0.260**), General Moral Concern for All AIs ($M_S$ = 0.261**), Protection Support ($M_M$ = 0.245**), LLM Suffering Concern ($M_S$ = 0.234**), General Moral Concern for Sentient AIs ($M_M$ = 0.248**), 100-Year Likelihood of Sentient AI ($M_M$ = 0.211**, $M_S$ = 0.197**), and Target-Specific Moral Concern ($M_M$ = 0.200**), as well as strongly predicting decreases in General Threat ($M_S$ = -0.145**), Slowdown Support ($M_S$ = -0.118**), and Ban Support ($M_S$ = -0.101*).

Increased age strongly predicted increases in Subservience ($M_M$ = 0.165**, $M_S$ = 0.148**) as well as decreases in Mind-Related Anthropomorphism ($M_M$ = -0.182**), Positive Emotions ($M_S$ = -0.174**), LLM Suffering Concern ($M_S$ = -0.168**), 100-Year Likelihood of Sentient AI ($M_S$ = -0.135**), General Mind Perception ($M_M$ = -0.134**), Trust ($M_S$ = -0.133**), LLM Mind Perception ($M_S$ = -0.124**), and Protection Support ($M_M$ = -0.114**).
 
Conservative political orientation strongly predicted increases in Ban Support ($M_M$ = 0.171**), General Threat ($M_M$ = 0.137**), Subservience ($M_S$ = 0.107**), and Existential Threat ($M_S$ = 0.107**) as well as decreases in General Moral Concern for Sentient AIs ($M_M$ = -0.121**), General Moral Concern for All AIs ($M_S$ = -0.106**), and LLM Suffering Concern ($M_S$ = -0.103**).

Male gender strongly predicted increases in Trust ($M_S$ = 0.156**) and Positive Emotions ($M_S$ = 0.147**) as well as decreases in Ban Support ($M_M$ = -0.138**, $M_S$ = -0.146**) and Slowdown Support ($M_S$ = -0.129**).

\bibliographystyle{ACM-Reference-Format}
\bibliography{references, supplemental_materials/references_supplement}

\end{document}
