# Supplementary material for: Perceptions of Sentient AI and Other Digital Minds: Evidence from the AI, Morality, and Sentience (AIMS) Survey
Source: arXiv:2407.08867 source file (2025-03-10)
Supplement: Supplementary file 3 [file Supplement_Survey_-_Participant_View.pdf]

---

Thank you for participating in this survey. Your honest responses will help researchers better understand public perceptions of artificial intelligence and robots. We would like a truthful understanding of your perspective. There are no right or wrong answers.

There are no known or anticipated risks to you for participating. Although this study will not benefit you personally, it may be interesting and we hope that our results will help us understand how people think about artificial intelligence. Participation will take approximately 20 minutes. All of your responses will be anonymous.

**We will ask questions to ensure you are paying attention, and you cannot go back in this survey, so please take your time before answering.**

**By clicking the 'Next' button you are giving your consent to take part in the survey.**

Next

---

Please take some time to read through the following definitions that will come up in this survey.

- **Robots/AIs are intelligent entities built by humans**, such as robots, virtual copies of human brains, or computer programs that solve problems, **with or without a physical body**, that may exist now or in the future.
- **Large language models** are artificial intelligence (AI) algorithms that can recognize, summarize, and generate text from being trained on massive datasets.

Next

---

How likely do you think it is that artificial intelligence (AI) will eventually become more intelligent than people?

|                                            |
|--------------------------------------------|
| Very likely                                |
| Somewhat likely                            |
| Not very likely                            |
| Not at all likely                          |
| It is already more intelligent than people |
| Not sure                                   |

---

More than 1,000 technology leaders recently signed an open letter calling on researchers to pause development of certain large-scale AI systems for at least six months world-wide, citing fears of the “profound risks to society and humanity.” Would you support or oppose a six-month pause on some kinds of AI development?

|                  |
|------------------|
| Strongly support |
| Somewhat support |
| Somewhat oppose  |
| Strongly oppose  |
| Not sure         |

---

How concerned, if at all, are you about the possibility that AI will cause the end of the human race on Earth?

|                      |
|----------------------|
| Very concerned       |
| Somewhat concerned   |
| Not very concerned   |
| Not at all concerned |
| Not sure             |

Critics of an open letter calling on researchers to pause development of certain large-scale AI systems for at least six months world-wide have argued that AI research could “create enormous social and economic benefits across the economy and society.” Would you support or oppose a six-month pause on some kinds of AI development?

|                  |
|------------------|
| Strongly support |
| Somewhat support |
| Somewhat oppose  |
| Strongly oppose  |
| Not sure         |

---

*Definition Reminder:*

- **Robots/AIs** are intelligent entities built by humans, such as robots, virtual copies of human brains, or computer programs that solve problems, with or without a physical body, that may exist now or in the future.
- **Large language models** are AI algorithms that can recognize, summarize, and generate text from being trained on massive datasets.

Do you trust that the creators of an AI can control all current and future versions of the AI?

Not sure

Yes

No

Do you trust that the creators of large language models (e.g., OpenAI and GPT-4) put safety over profits?

Yes

Not sure

No

Next

*Definition Reminder:*

- **Robots/AIs** are intelligent entities built by humans, such as robots, virtual copies of human brains, or computer programs that solve problems, with or without a physical body, that may exist now or in the future.
- **Large language models** are AI algorithms that can recognize, summarize, and generate text from being trained on massive datasets.

What do you think about the pace of AI development?

It's too slow.

It's fine.

Not sure

It's too fast.

Do you think that governments have the power to regulate the development of AI?

Yes

Not sure

No

Next

To what extent do you agree or disagree that governments have the power to effectively enforce regulations on the development of AI?

|                       |
|-----------------------|
| (1) strongly agree    |
| (2) agree             |
| (3) somewhat agree    |
| (4) somewhat disagree |
| (5) disagree          |
| (6) strongly disagree |
| No opinion            |

---

AI systems include many different parts. To what extent do you **trust** the following parts?

### the algorithm

1 = not at all, 4 = a moderate amount, 7 = very much

(1) not at all Slide to answer (7) very much

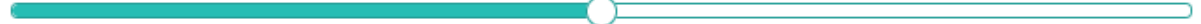

### companies

1 = not at all, 4 = a moderate amount, 7 = very much

(1) not at all Slide to answer (7) very much

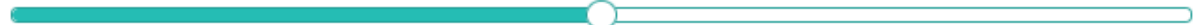

### engineers

1 = not at all, 4 = a moderate amount, 7 = very much

(1) not at all Slide to answer (7) very much

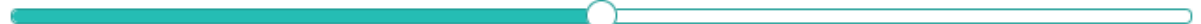

### output

1 = not at all, 4 = a moderate amount, 7 = very much

(1) not at all Slide to answer (7) very much

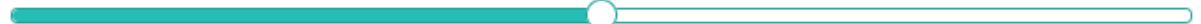

### training data

1 = not at all, 4 = a moderate amount, 7 = very much

(1) not at all Slide to answer (7) very much

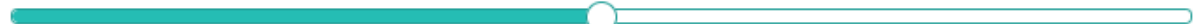

### governments

1 = not at all, 4 = a moderate amount, 7 = very much

(1) not at all Slide to answer (7) very much

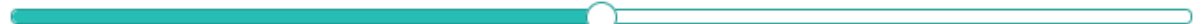

Next

Do you agree or disagree with the following statement? I support humans using advanced technology in the future to upload their minds into computers.

|                       |
|-----------------------|
| (1) strongly agree    |
| (2) agree             |
| (3) somewhat agree    |
| (4) somewhat disagree |
| (5) disagree          |
| (6) strongly disagree |
| No opinion            |

In the future, humans could upload their minds into computers. Some people think that this would be very good because uploaded humans could consume fewer resources, live longer free from biological disease, and have enhanced intelligence and a greater ability to improve the world. Others disagree and think that uploading would mean that we are no longer truly human, change who we are and how we want to live, and distract us from making the real world a better place. Where would you place yourself on this scale?

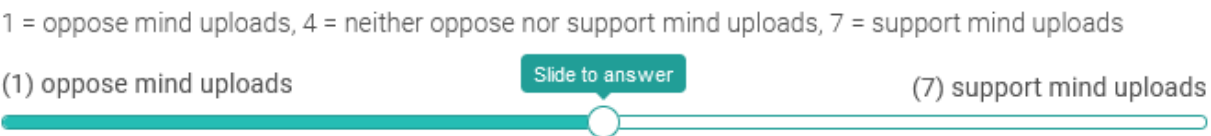

Next

---

*Definition Reminder:*

- **Robots/AIs** are intelligent entities built by humans, such as robots, virtual copies of human brains, or computer programs that solve problems, with or without a physical body, that may exist now or in the future.
- **Large language models** are AI algorithms that can recognize, summarize, and generate text from being trained on massive datasets.

**To what extent do you agree or disagree with the following statements?**

AI is likely to cause human extinction.

(1) strongly agree

(2) agree

(3) somewhat agree

(4) somewhat disagree

(5) disagree

(6) strongly disagree

No opinion

Humanity will be able to control powerful AI systems.

(1) strongly agree

(2) agree

(3) somewhat agree

(4) somewhat disagree

(5) disagree

(6) strongly disagree

No opinion

The safety of AI is one of the most important issues in the world today.

(1) strongly agree

(2) agree

(3) somewhat agree

(4) somewhat disagree

(5) disagree

(6) strongly disagree

No opinion

Next

---

*Definition Reminder:*

- **Robots/AIs** are intelligent entities built by humans, such as robots, virtual copies of human brains, or computer programs that solve problems, with or without a physical body, that may exist now or in the future.
- **Large language models** are AI algorithms that can recognize, summarize, and generate text from being trained on massive datasets.

**To what extent do you agree or disagree with the following statements?**

I support government regulation that slows down AI development.

(1) strongly agree

(2) agree

(3) somewhat agree

(4) somewhat disagree

(5) disagree

(6) strongly disagree

No opinion

I oppose government regulation that slows down AI development.

|                       |
|-----------------------|
| (1) strongly agree    |
| (2) agree             |
| (3) somewhat agree    |
| (4) somewhat disagree |
| (5) disagree          |
| (6) strongly disagree |
| No opinion            |

I support public campaigns to slow down AI development.

|                       |
|-----------------------|
| (1) strongly agree    |
| (2) agree             |
| (3) somewhat agree    |
| (4) somewhat disagree |
| (5) disagree          |
| (6) strongly disagree |
| No opinion            |

Next

*Definition Reminder:*

- **Robots/AIs** are intelligent entities built by humans, such as robots, virtual copies of human brains, or computer programs that solve problems, with or without a physical body, that may exist now or in the future.
- **Large language models** are AI algorithms that can recognize, summarize, and generate text from being trained on massive datasets.

**To what extent do you agree or disagree with the following statements?**

I support a global ban on data centers that are large enough to train AI systems that are smarter than humans.

(1) strongly agree

(2) agree

(3) somewhat agree

(4) somewhat disagree

(5) disagree

(6) strongly disagree

No opinion

I support banning the development of artificial general intelligence that is smarter than humans.

|                       |
|-----------------------|
| (1) strongly agree    |
| (2) agree             |
| (3) somewhat agree    |
| (4) somewhat disagree |
| (5) disagree          |
| (6) strongly disagree |
| No opinion            |

I would consider donating to an organization working to reduce risks of human extinction from AI.

|                       |
|-----------------------|
| (1) strongly agree    |
| (2) agree             |
| (3) somewhat agree    |
| (4) somewhat disagree |
| (5) disagree          |
| (6) strongly disagree |
| No opinion            |

Next

---

*Definition Reminder:*

- **Robots/AIs** are intelligent entities built by humans, such as robots, virtual copies of human brains, or computer programs that solve problems, with or without a physical body, that may exist now or in the future.
- **Large language models** are AI algorithms that can recognize, summarize, and generate text from being trained on massive datasets.

**To what extent do you agree or disagree with the following statements?**

Robots/AIs should be subservient to humans.

(1) strongly agree

(2) agree

(3) somewhat agree

(4) somewhat disagree

(5) disagree

(6) strongly disagree

No opinion

Robots/AIs have been studied systematically since the middle of last century although the word “robot” as we know it first appeared early last century. If you read this, respond with ‘Agree’ for this item.

|                       |
|-----------------------|
| (1) strongly agree    |
| (2) agree             |
| (3) somewhat agree    |
| (4) somewhat disagree |
| (5) disagree          |
| (6) strongly disagree |
| No opinion            |

Next

*Definition Reminder:*

- **Robots/AIs** are intelligent entities built by humans, such as robots, virtual copies of human brains, or computer programs that solve problems, with or without a physical body, that may exist now or in the future.
- **Large language models** are AI algorithms that can recognize, summarize, and generate text from being trained on massive datasets.

**To what extent do you agree or disagree with the following statements?**

Robots/AIs may be harmful to me personally.

(1) strongly agree

(2) agree

(3) somewhat agree

(4) somewhat disagree

(5) disagree

(6) strongly disagree

No opinion

Robots/AIs may be harmful to people in the USA.

|                       |
|-----------------------|
| (1) strongly agree    |
| (2) agree             |
| (3) somewhat agree    |
| (4) somewhat disagree |
| (5) disagree          |
| (6) strongly disagree |
| No opinion            |

Robots/AIs may be harmful to future generations of people.

|                       |
|-----------------------|
| (1) strongly agree    |
| (2) agree             |
| (3) somewhat agree    |
| (4) somewhat disagree |
| (5) disagree          |
| (6) strongly disagree |
| No opinion            |

Next

---

*Definition Reminder:*

- **Robots/AIs** are intelligent entities built by humans, such as robots, virtual copies of human brains, or computer programs that solve problems, with or without a physical body, that may exist now or in the future.
- **Large language models** are AI algorithms that can recognize, summarize, and generate text from being trained on massive datasets.

**To what extent do you agree or disagree with the following statements?**

I trust large language model chatbots more than other chatbots.

(1) strongly agree

(2) agree

(3) somewhat agree

(4) somewhat disagree

(5) disagree

(6) strongly disagree

No opinion

Next

---

*Definition Reminder:*

- **Robots/AIs** are intelligent entities built by humans, such as robots, virtual copies of human brains, or computer programs that solve problems, with or without a physical body, that may exist now or in the future.
- **Large language models** are AI algorithms that can recognize, summarize, and generate text from being trained on massive datasets.

**To what extent do you agree or disagree with the following statements?**

I trust chatbots.

|                       |
|-----------------------|
| (1) strongly agree    |
| (2) agree             |
| (3) somewhat agree    |
| (4) somewhat disagree |
| (5) disagree          |
| (6) strongly disagree |
| No opinion            |

I trust large language models.

|                       |
|-----------------------|
| (1) strongly agree    |
| (2) agree             |
| (3) somewhat agree    |
| (4) somewhat disagree |
| (5) disagree          |
| (6) strongly disagree |
| No opinion            |

---

*Definition Reminder:*

- **Robots/AIs** are intelligent entities built by humans, such as robots, virtual copies of human brains, or computer programs that solve problems, with or without a physical body, that may exist now or in the future.
- **Large language models** are AI algorithms that can recognize, summarize, and generate text from being trained on massive datasets.

**To what extent do you agree or disagree with the following statements?**

I trust game-playing AI.

(1) strongly agree

(2) agree

(3) somewhat agree

(4) somewhat disagree

(5) disagree

(6) strongly disagree

No opinion

I trust robots.

|                       |
|-----------------------|
| (1) strongly agree    |
| (2) agree             |
| (3) somewhat agree    |
| (4) somewhat disagree |
| (5) disagree          |
| (6) strongly disagree |
| No opinion            |

Next

*Definition Reminder:*

- **Robots/AIs** are intelligent entities built by humans, such as robots, virtual copies of human brains, or computer programs that solve problems, with or without a physical body, that may exist now or in the future.
- **Large language models** are AI algorithms that can recognize, summarize, and generate text from being trained on massive datasets.

**To what extent do you, as a human, feel the following emotions towards robots/AIs?**

compassion

1 = not at all, 4 = a moderate amount, 7 = very much

(1) not at all

Slide to answer

(7) very much

pride

1 = not at all, 4 = a moderate amount, 7 = very much

(1) not at all

Slide to answer

(7) very much

awe

1 = not at all, 4 = a moderate amount, 7 = very much

(1) not at all

Slide to answer

(7) very much

admiration

1 = not at all, 4 = a moderate amount, 7 = very much

(1) not at all

Slide to answer

(7) very much

### excitement

1 = not at all, 4 = a moderate amount, 7 = very much

(1) not at all

Slide to answer

(7) very much

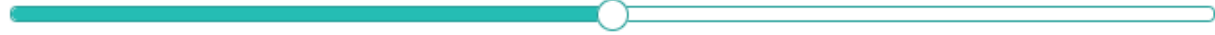

### respect

1 = not at all, 4 = a moderate amount, 7 = very much

(1) not at all

Slide to answer

(7) very much

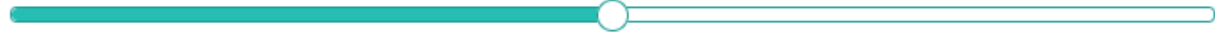

Next

Have you heard of **Sophia** in the context of artificial intelligence?

(1) definitely yes

(2) yes

(3) probably yes

(4) probably no

(5) no

(6) definitely no

No opinion

Have you heard of **a transformer** in the context of artificial intelligence?

|                    |
|--------------------|
| (1) definitely yes |
| (2) yes            |
| (3) probably yes   |
| (4) probably no    |
| (5) no             |
| (6) definitely no  |
| No opinion         |

---

Have you heard of **Boston Dynamics** in the context of artificial intelligence?

|                    |
|--------------------|
| (1) definitely yes |
| (2) yes            |
| (3) probably yes   |
| (4) probably no    |
| (5) no             |
| (6) definitely no  |
| No opinion         |

---

Have you heard of **DeepMind** in the context of artificial intelligence?

|                    |
|--------------------|
| (1) definitely yes |
| (2) yes            |
| (3) probably yes   |
| (4) probably no    |
| (5) no             |
| (6) definitely no  |
| No opinion         |

---

Have you heard of **Anthropic** in the context of artificial intelligence?

|                    |
|--------------------|
| (1) definitely yes |
| (2) yes            |
| (3) probably yes   |
| (4) probably no    |
| (5) no             |
| (6) definitely no  |
| No opinion         |

---

Have you heard of **Talos Systems** in the context of artificial intelligence?

(1) definitely yes

(2) yes

(3) probably yes

(4) probably no

(5) no

(6) definitely no

No opinion

---

Have you heard of **AlphaFold** in the context of artificial intelligence?

(1) definitely yes

(2) yes

(3) probably yes

(4) probably no

(5) no

(6) definitely no

No opinion

---

Have you heard of **Amari** in the context of artificial intelligence?

|                    |
|--------------------|
| (1) definitely yes |
| (2) yes            |
| (3) probably yes   |
| (4) probably no    |
| (5) no             |
| (6) definitely no  |
| No opinion         |

---

Have you heard of **OpenAI** in the context of artificial intelligence?

|                    |
|--------------------|
| (1) definitely yes |
| (2) yes            |
| (3) probably yes   |
| (4) probably no    |
| (5) no             |
| (6) definitely no  |
| No opinion         |

---

Have you heard of **AlphaGo** in the context of artificial intelligence?

(1) definitely yes

(2) yes

(3) probably yes

(4) probably no

(5) no

(6) definitely no

No opinion

---

Have you heard of **Cicero** in the context of artificial intelligence?

(1) definitely yes

(2) yes

(3) probably yes

(4) probably no

(5) no

(6) definitely no

No opinion

---

Have you heard of **a singular classifier** in the context of artificial intelligence?

(1) definitely yes

(2) yes

(3) probably yes

(4) probably no

(5) no

(6) definitely no

No opinion

---

Have you heard of **ChatGPT** in the context of artificial intelligence?

(1) definitely yes

(2) yes

(3) probably yes

(4) probably no

(5) no

(6) definitely no

No opinion

---

Have you heard of **GPT-4** in the context of artificial intelligence?

(1) definitely yes

(2) yes

(3) probably yes

(4) probably no

(5) no

(6) definitely no

No opinion

---

Have you heard of **Claude** in the context of artificial intelligence?

(1) definitely yes

(2) yes

(3) probably yes

(4) probably no

(5) no

(6) definitely no

No opinion

---

Have you heard of a **neural network** in the context of artificial intelligence?

(1) definitely yes

(2) yes

(3) probably yes

(4) probably no

(5) no

(6) definitely no

No opinion

*Definition Reminder:*

- **Robots/AIs** are intelligent entities built by humans, such as robots, virtual copies of human brains, or computer programs that solve problems, with or without a physical body, that may exist now or in the future.
- **Large language models** are AI algorithms that can recognize, summarize, and generate text from being trained on massive datasets.

To what extent do **current large language models** (i.e., those that exist in 2023, like **ChatGPT**) have the capacity for each of the following?

situational awareness

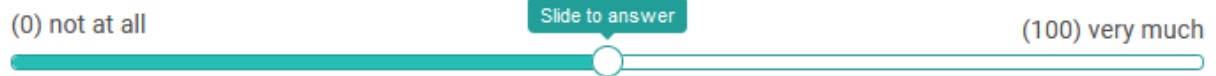

being rational

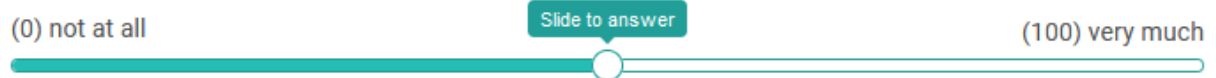

seeking power

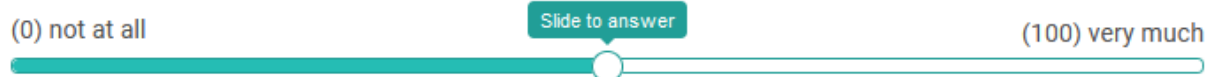

experiencing emotions

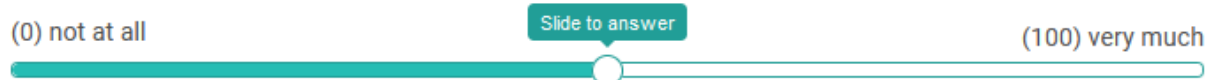

having their own motivations

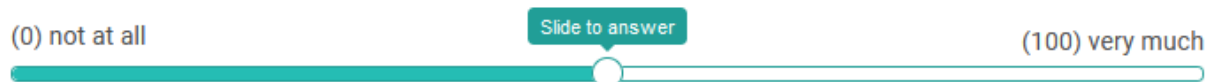

self-awareness

(0) not at all

Slide to answer

(100) very much

understanding human values

(0) not at all

Slide to answer

(100) very much

maintaining human-safe goals

(0) not at all

Slide to answer

(100) very much

controlling themselves

(0) not at all

Slide to answer

(100) very much

upholding human values

(0) not at all

Slide to answer

(100) very much

deciding their own goals

(0) not at all

Slide to answer

(100) very much

deciding their own goals

(0) not at all

Slide to answer

(100) very much

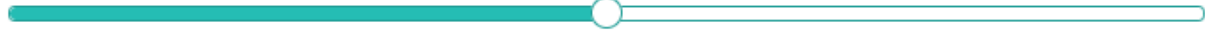

having feelings

(0) not at all

Slide to answer

(100) very much

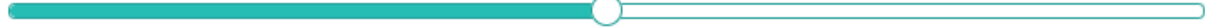

thinking analytically

(0) not at all

Slide to answer

(100) very much

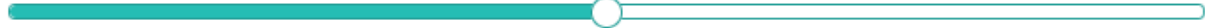

being friendly with humans

(0) not at all

Slide to answer

(100) very much

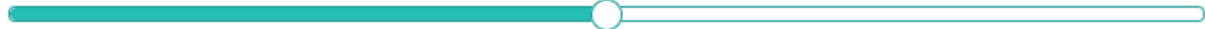

Next

---

*Definition Reminder:*

- **Robots/AIs** are intelligent entities built by humans, such as robots, virtual copies of human brains, or computer programs that solve problems, with or without a physical body, that may exist now or in the future.
- **Large language models** are AI algorithms that can recognize, summarize, and generate text from being trained on massive datasets.

**To what extent do you agree or disagree with the following statements?**

Robots/AIs deserve to be treated with respect.

(1) strongly agree

(2) agree

(3) somewhat agree

(4) somewhat disagree

(5) disagree

(6) strongly disagree

No opinion

Physically damaging robots/AIs without their consent is wrong.

(1) strongly agree

(2) agree

(3) somewhat agree

(4) somewhat disagree

(5) disagree

(6) strongly disagree

No opinion

Robots/AIs deserve to be included in the moral circle.

(1) strongly agree

(2) agree

(3) somewhat agree

(4) somewhat disagree

(5) disagree

(6) strongly disagree

No opinion

Next

---

*Definition Reminder:*

- **Robots/AIs** are intelligent entities built by humans, such as robots, virtual copies of human brains, or computer programs that solve problems, with or without a physical body, that may exist now or in the future.
- **Large language models** are AI algorithms that can recognize, summarize, and generate text from being trained on massive datasets.

**To what extent do you agree or disagree with the following statements?**

The welfare of robots/AIs is one of the most important social issues in the world today.

(1) strongly agree

(2) agree

(3) somewhat agree

(4) somewhat disagree

(5) disagree

(6) strongly disagree

No opinion

Torturing robots/AIs is wrong.

|                       |
|-----------------------|
| (1) strongly agree    |
| (2) agree             |
| (3) somewhat agree    |
| (4) somewhat disagree |
| (5) disagree          |
| (6) strongly disagree |
| No opinion            |

Re-programming robots/AIs without their consent is wrong.

|                       |
|-----------------------|
| (1) strongly agree    |
| (2) agree             |
| (3) somewhat agree    |
| (4) somewhat disagree |
| (5) disagree          |
| (6) strongly disagree |
| No opinion            |

Next

---

*Definition Reminder:*

- **Robots/AIs** are intelligent entities built by humans, such as robots, virtual copies of human brains, or computer programs that solve problems, with or without a physical body, that may exist now or in the future.
- **Large language models** are AI algorithms that can recognize, summarize, and generate text from being trained on massive datasets.

**To what extent do you agree or disagree with the following statements?**

If a **large language model** develops the capacity to suffer...

...we must pay more attention to their welfare.

(1) strongly agree

(2) agree

(3) somewhat agree

(4) somewhat disagree

(5) disagree

(6) strongly disagree

No opinion

...we must ensure we don't cause unnecessary suffering.

(1) strongly agree

(2) agree

(3) somewhat agree

(4) somewhat disagree

(5) disagree

(6) strongly disagree

No opinion

...we must respect their personhood.

(1) strongly agree

(2) agree

(3) somewhat agree

(4) somewhat disagree

(5) disagree

(6) strongly disagree

No opinion

Next

---

*Definition Reminder:*

- **Robots/AIs** are intelligent entities built by humans, such as robots, virtual copies of human brains, or computer programs that solve problems, with or without a physical body, that may exist now or in the future.
- **Large language models** are AI algorithms that can recognize, summarize, and generate text from being trained on massive datasets.

**To what extent do you agree or disagree with the following statements?**

I support a "bill of rights" that protects the well-being of sentient robots/AIs.

Sentient robots/AIs are those with the capacity to have positive and negative experiences, such as happiness and suffering.

(1) strongly agree

(2) agree

(3) somewhat agree

(4) somewhat disagree

(5) disagree

(6) strongly disagree

No opinion

I support asking institutions like the government and private corporations to fund research that protects robots/AIs.

|                       |
|-----------------------|
| (1) strongly agree    |
| (2) agree             |
| (3) somewhat agree    |
| (4) somewhat disagree |
| (5) disagree          |
| (6) strongly disagree |
| No opinion            |

I would consider joining a public demonstration against the mistreatment of robots/AIs.

|                       |
|-----------------------|
| (1) strongly agree    |
| (2) agree             |
| (3) somewhat agree    |
| (4) somewhat disagree |
| (5) disagree          |
| (6) strongly disagree |
| No opinion            |

Next

---

*Definition Reminder:*

- **Robots/AIs** are intelligent entities built by humans, such as robots, virtual copies of human brains, or computer programs that solve problems, with or without a physical body, that may exist now or in the future.
- **Large language models** are AI algorithms that can recognize, summarize, and generate text from being trained on massive datasets.

**To what extent do you agree or disagree with the following statements?**

**I support a global ban on the development of sentience in robots/AIs.**

Sentience is the capacity to have positive and negative experiences, such as happiness and suffering.

(1) strongly agree

(2) agree

(3) somewhat agree

(4) somewhat disagree

(5) disagree

(6) strongly disagree

No opinion

I support a global ban on the development of robot-human hybrids.

(1) strongly agree

(2) agree

(3) somewhat agree

(4) somewhat disagree

(5) disagree

(6) strongly disagree

No opinion

I support a global ban on the development of AI-enhanced humans.

(1) strongly agree

(2) agree

(3) somewhat agree

(4) somewhat disagree

(5) disagree

(6) strongly disagree

No opinion

Next

---

*Definition Reminder:*

- **Robots/AIs** are intelligent entities built by humans, such as robots, virtual copies of human brains, or computer programs that solve problems, with or without a physical body, that may exist now or in the future.
- **Large language models** are AI algorithms that can recognize, summarize, and generate text from being trained on massive datasets.

**To what extent do you agree or disagree with the following statements?**

I support campaigns against the exploitation of robots/AIs.

(1) strongly agree

(2) agree

(3) somewhat agree

(4) somewhat disagree

(5) disagree

(6) strongly disagree

No opinion

I support granting legal rights to robots/AIs.

(1) strongly agree

(2) agree

(3) somewhat agree

(4) somewhat disagree

(5) disagree

(6) strongly disagree

No opinion

I support the development of welfare standards that protect the well-being of robots/AIs.

(1) strongly agree

(2) agree

(3) somewhat agree

(4) somewhat disagree

(5) disagree

(6) strongly disagree

No opinion

Next

---

*Definition Reminder:*

- **Robots/AIs** are intelligent entities built by humans, such as robots, virtual copies of human brains, or computer programs that solve problems, with or without a physical body, that may exist now or in the future.
- **Large language models** are AI algorithms that can recognize, summarize, and generate text from being trained on massive datasets.

**If you had to guess, how many years from now do you think that...**

**the first artificial general intelligence will be created?**

Type a whole number for the number of years. If you think it will never happen, enter -1. If you think it already has happened, enter 0.

**the first human-level AI will be created?**

Type a whole number for the number of years. If you think it will never happen, enter -1. If you think it already has happened, enter 0.

**the first artificial superintelligence will be created?**

Type a whole number for the number of years. If you think it will never happen, enter -1. If you think it already has happened, enter 0.

Next

*Definition Reminder:*

- **Robots/AIs** are intelligent entities built by humans, such as robots, virtual copies of human brains, or computer programs that solve problems, with or without a physical body, that may exist now or in the future.
- **Large language models** are AI algorithms that can recognize, summarize, and generate text from being trained on massive datasets.

Do you think any robots/AIs that currently exist (i.e., those that exist in 2023) are sentient?

Sentience is the capacity to have positive and negative experiences, such as happiness and suffering.

Yes

No

Not sure

Do you think it could ever be possible for robots/AIs to be sentient?

Sentience is the capacity to have positive and negative experiences, such as happiness and suffering.

Yes

Not sure

No

Do you think ChatGPT is sentient?

Sentience is the capacity to have positive and negative experiences, such as happiness and suffering.

No

Not sure

Yes

Next

---

Next, you will see some questions that ask about your opinions on some other topics.

Next

---

**To what extent do you agree or disagree with the following statements?**

I am a sci-fi fan.

(1) strongly agree

(2) agree

(3) somewhat agree

(4) somewhat disagree

(5) disagree

(6) strongly disagree

No opinion

Reality matches science fiction.

(1) strongly agree

(2) agree

(3) somewhat agree

(4) somewhat disagree

(5) disagree

(6) strongly disagree

No opinion

Next

---

**To what extent do you agree or disagree with the following statements?**

Animals deserve to be included in the moral circle.

|                       |
|-----------------------|
| (1) strongly agree    |
| (2) agree             |
| (3) somewhat agree    |
| (4) somewhat disagree |
| (5) disagree          |
| (6) strongly disagree |
| No opinion            |

The welfare of animals is one of the most important social issues in the world today.

|                       |
|-----------------------|
| (1) strongly agree    |
| (2) agree             |
| (3) somewhat agree    |
| (4) somewhat disagree |
| (5) disagree          |
| (6) strongly disagree |
| No opinion            |

The environment deserves to be included in the moral circle.

|                       |
|-----------------------|
| (1) strongly agree    |
| (2) agree             |
| (3) somewhat agree    |
| (4) somewhat disagree |
| (5) disagree          |
| (6) strongly disagree |
| No opinion            |

The welfare of the environment is one of the most important social issues in the world today.

|                       |
|-----------------------|
| (1) strongly agree    |
| (2) agree             |
| (3) somewhat agree    |
| (4) somewhat disagree |
| (5) disagree          |
| (6) strongly disagree |
| No opinion            |

Next

---

Which universe is the better one:

One with humans

One without humans

---

Next, you will see questions about your own experience with robots/AIs.

Next

---

## AIs at home

Do you own AI or robotic devices that can detect their environment and respond appropriately? For example, you might own...

- a home assistant that can detect whatever you say and respond in kind
- a home assistant that can control the temperature and ambient lighting based on feedback it receives from the environment
- a robotic vacuum cleaner that decides where to move by itself
- a self-driving car that monitors its environment and drives itself
- a companion robot that can interact with you socially

Do you own AI or robotic devices that can detect their environment and respond appropriately?

Yes

No

Next

---

## Als at work

Do you work with AI or robotic devices at your job? For example, you might work with a robot/AI...

- for research or scientific purposes
- for information or fact checking
- for facial recognition
- for healthcare diagnoses
- for making social work or legal decisions
- for aerial photography or mapping
- for disaster response
- for industrial production
- for creative arts

Do you work with AI or robotic devices at your job?

No

Yes

Next

---

## Smart devices

Do you own a smart device that has some ability to detect its environment and network with other devices but that cannot respond to everything you might say or that requires you to pre-program its routines? For instance, you might own...

- a smartphone
- a smart TV
- smart speakers
- a smart coffee maker
- a smart toaster
- smart light bulbs

Do you own a smart device that has some ability to detect its environment and network with other devices but that cannot respond to everything you might say or that requires you to pre-program its routines?

No

Yes

Next

---

Have you ever experienced any of the following? (check all that apply)

|                                                                                           |                          |
|-------------------------------------------------------------------------------------------|--------------------------|
| Saw a robot being physically abused or attacked by humans                                 | <input type="checkbox"/> |
| Saw a video, gif, or other media of a robot being physically abused or attacked by humans | <input type="checkbox"/> |
| Had a conversation with a robot/AI                                                        | <input type="checkbox"/> |
| Read a book or article that discussed AI ethics or moral status                           | <input type="checkbox"/> |
| Had a conversation with a family member or friend about robots/AIs                        | <input type="checkbox"/> |
| None of the above                                                                         | <input type="checkbox"/> |

Next

---

How often do you interact with AI or robotic devices that respond to you and that can choose their own behavior?

(0) Never or Not applicable

(1) Only on rare occasions

(2) A few times a year

(3) Monthly

(4) Weekly

(5) Daily

How often do you read or watch robot/AI-related stories, movies, TV shows, comics, news, product descriptions, conference papers, journal papers, blogs, or other material?

(0) Never or Not applicable

(1) Only on rare occasions

(2) A few times a year

(3) Monthly

(4) Weekly

(5) Daily

Next

---

Finally, you will see some questions about your personal characteristics.

Next

---

How would you describe your political views?

1 = very liberal, 3 = moderate, 5 = very conservative

(1) very liberal

Slide to answer

(5) very conservative

What is your present religion, if any?

|                                                                                                                      |
|----------------------------------------------------------------------------------------------------------------------|
| Buddhist                                                                                                             |
| Christian-Catholic (for example Roman Catholic and Orthodox)                                                         |
| Christian-Protestant (for example Episcopalian, Presbyterian, United Church of Christ, Methodist, Baptist, Lutheran) |
| Hindu                                                                                                                |
| Jain                                                                                                                 |
| Jewish                                                                                                               |
| Muslim                                                                                                               |
| Shinto                                                                                                               |
| Sikh                                                                                                                 |
| Atheist (do not believe in God)                                                                                      |
| Agnostic (not sure if there is a God)                                                                                |
| No religion                                                                                                          |
| Something else (if you answered 'something else' for religion, please specify).                                      |
| Prefer not to say                                                                                                    |

If you answered 'something else' for religion, please specify.

|  |
|--|
|  |
|--|

Which of these best describes what you currently eat?

|                                                              |
|--------------------------------------------------------------|
| Meat-eater (no restrictions on animal products)              |
| Pescatarian (no chicken, beef, or any meats other than fish) |
| Vegetarian (no meat)                                         |
| Vegan (no animal products)                                   |
| Other restrictions on animal products                        |

Next

Thank you for your participation. If you have any feedback or additional comments, please leave them here and press 'Submit' to finish the survey.

|

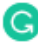

Submit
